# Supplementary material for: Scaling in Internet Traffic: a 14 year and 3 day longitudinal study, with multiscale analyses and random projections
Source: arXiv:1703.02005 source file (2017-03-06)
Supplement: Supplementary file 1 [file supplementary.tex]

\begin{figure*}
\centerline{
 \includegraphics[width=0.5\linewidth]{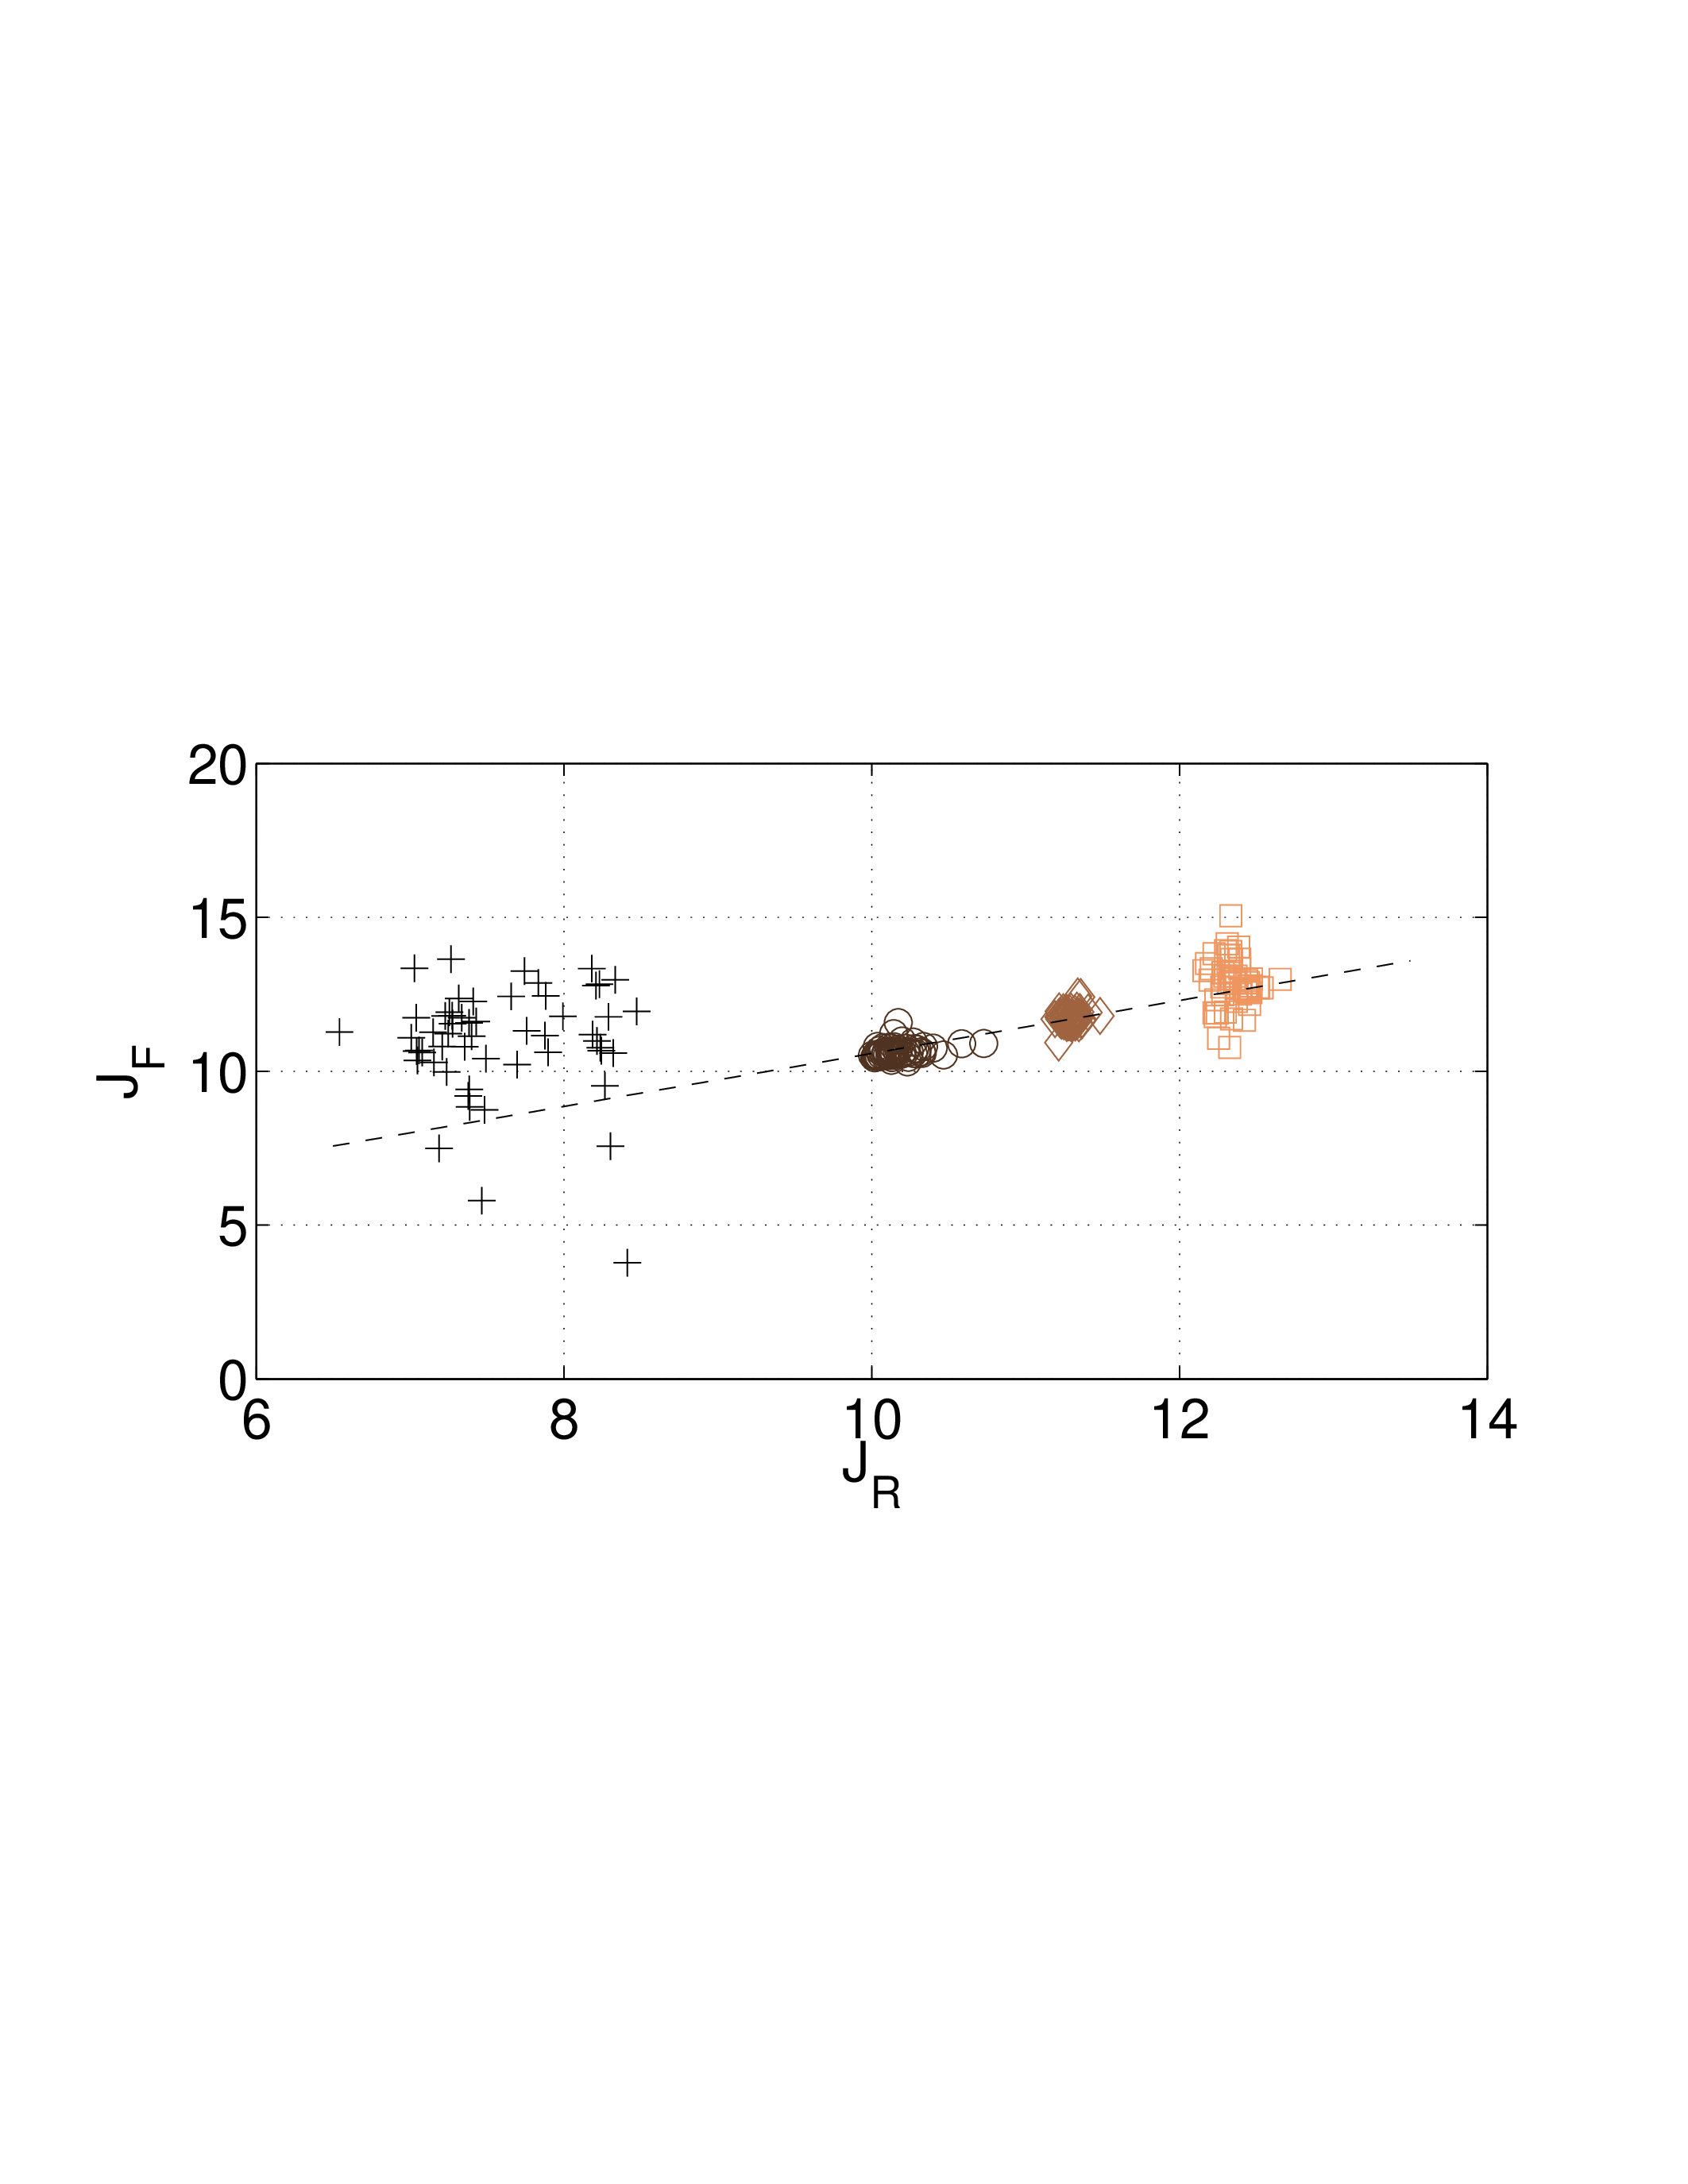}
  \includegraphics[width=0.5\linewidth]{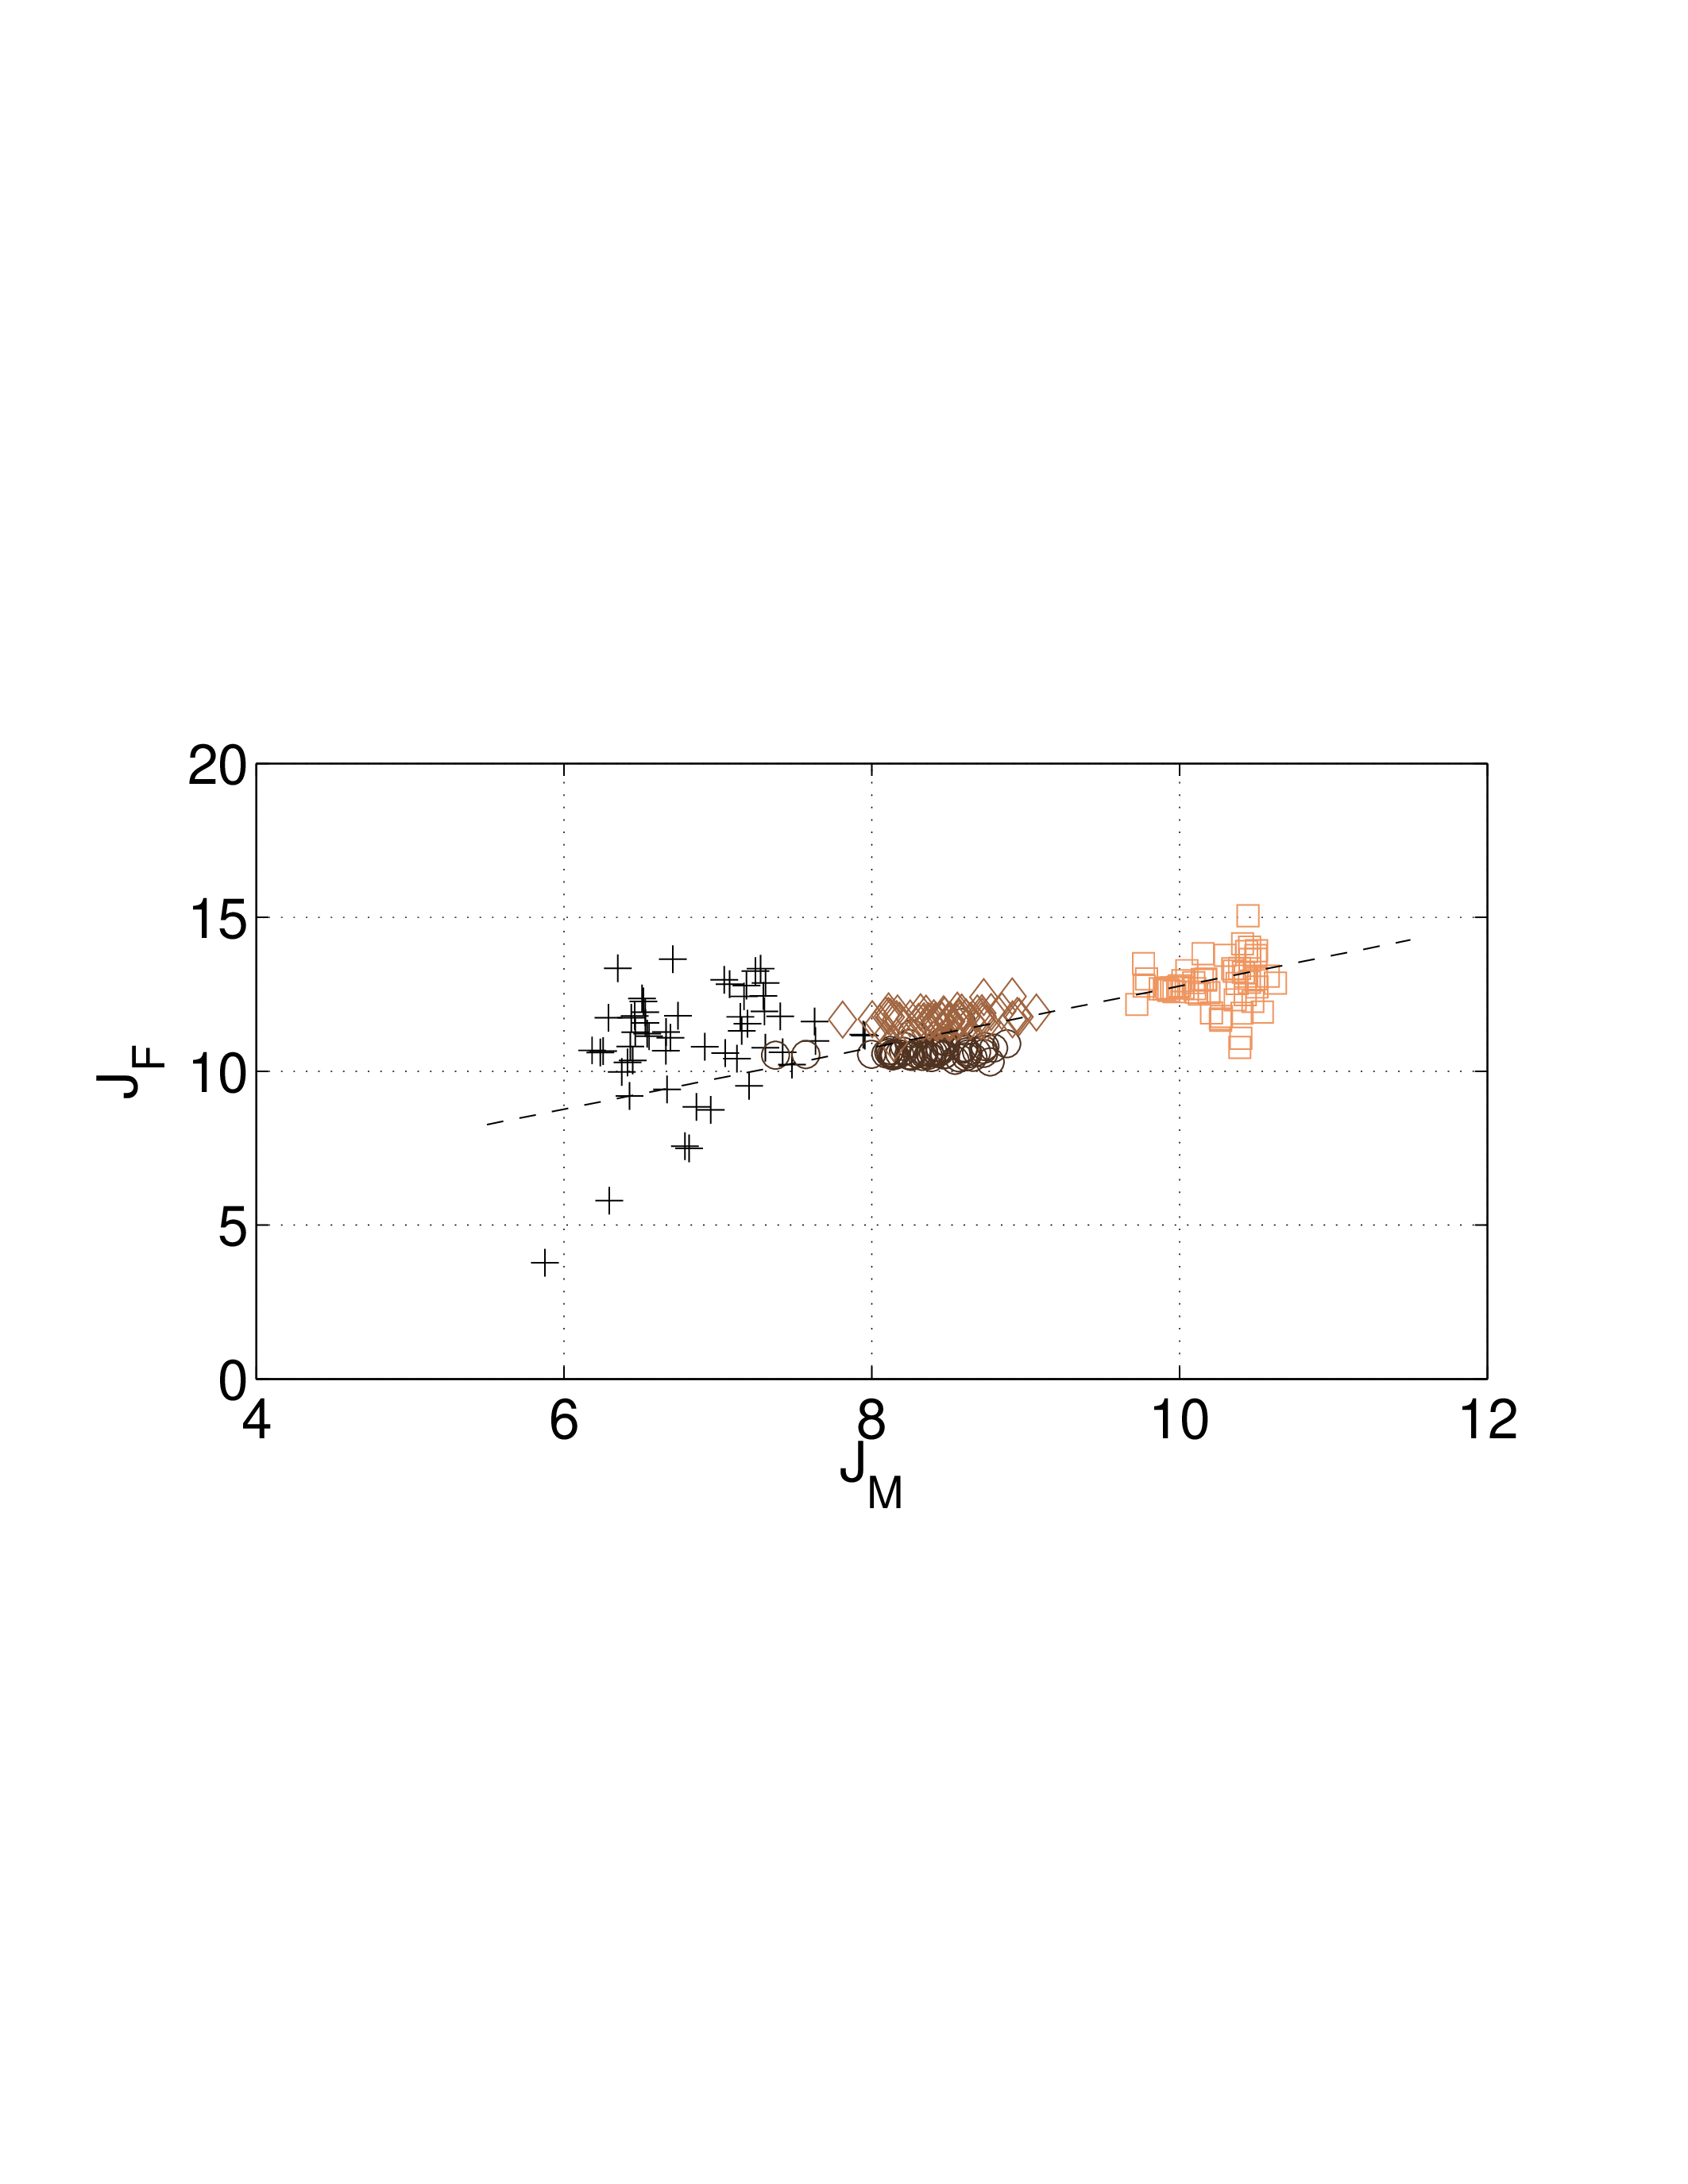}
}
\centerline{
  \includegraphics[width=0.5\linewidth]{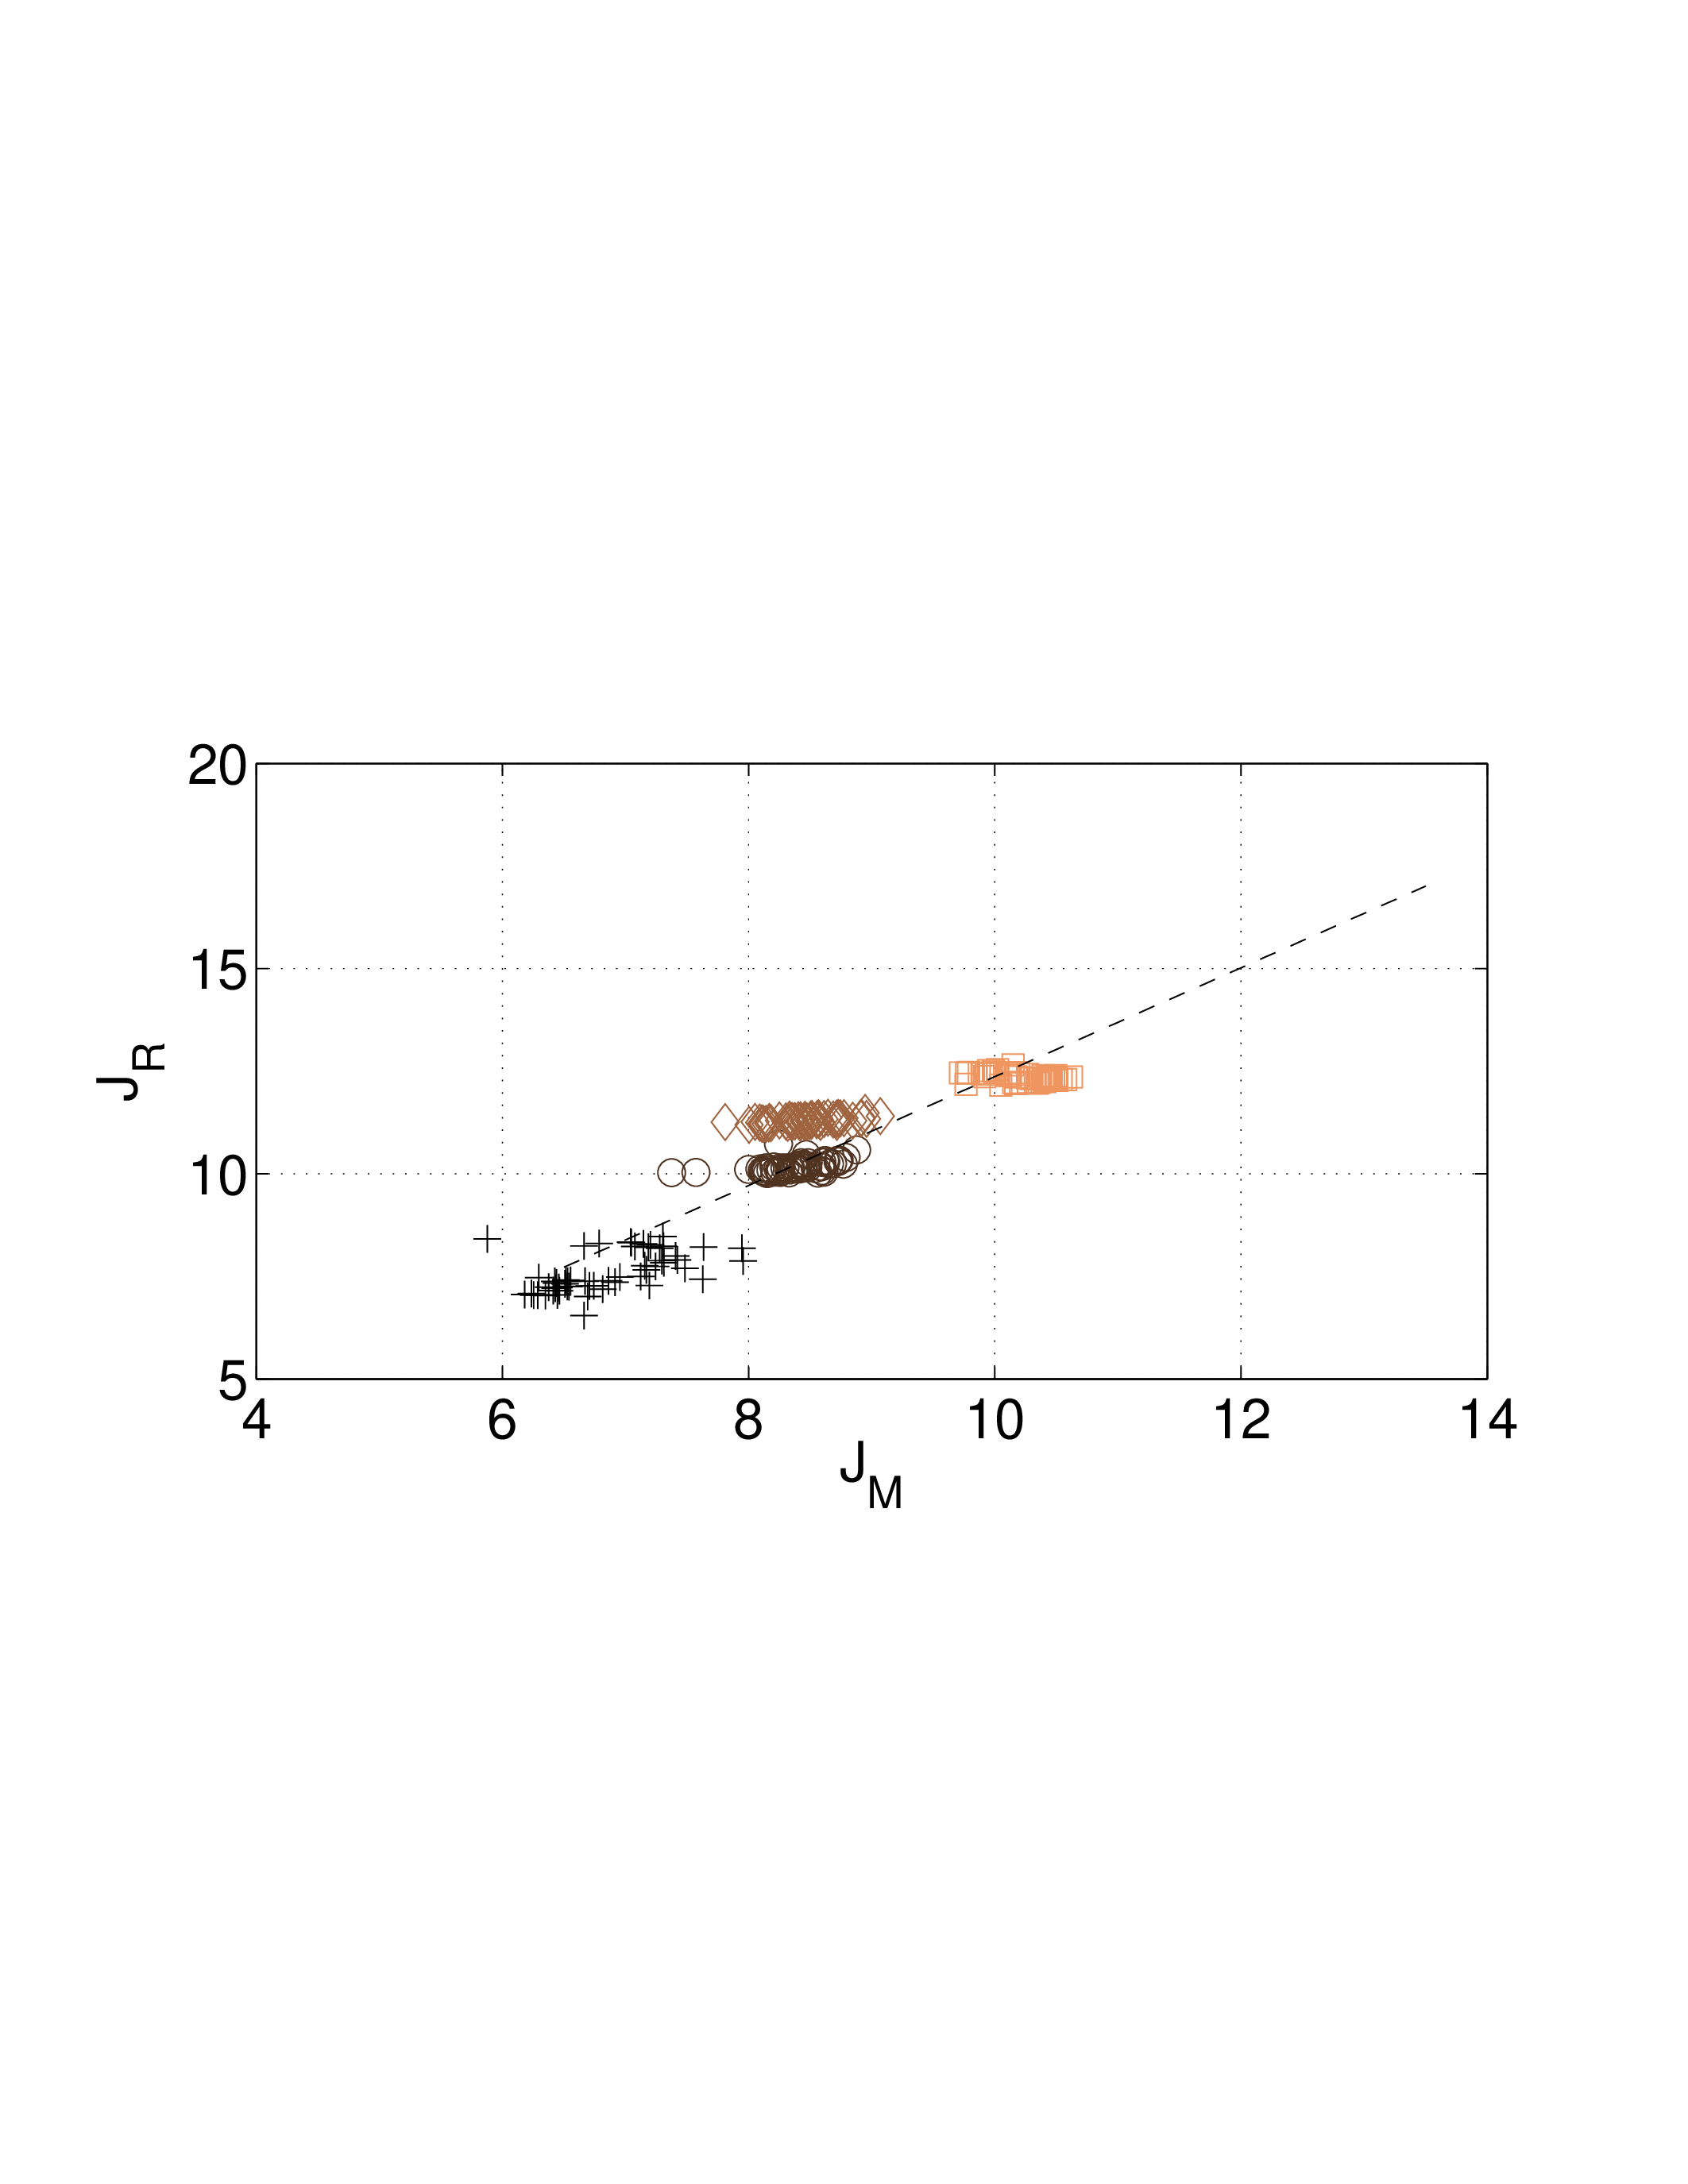}
   \includegraphics[width=0.5\linewidth]{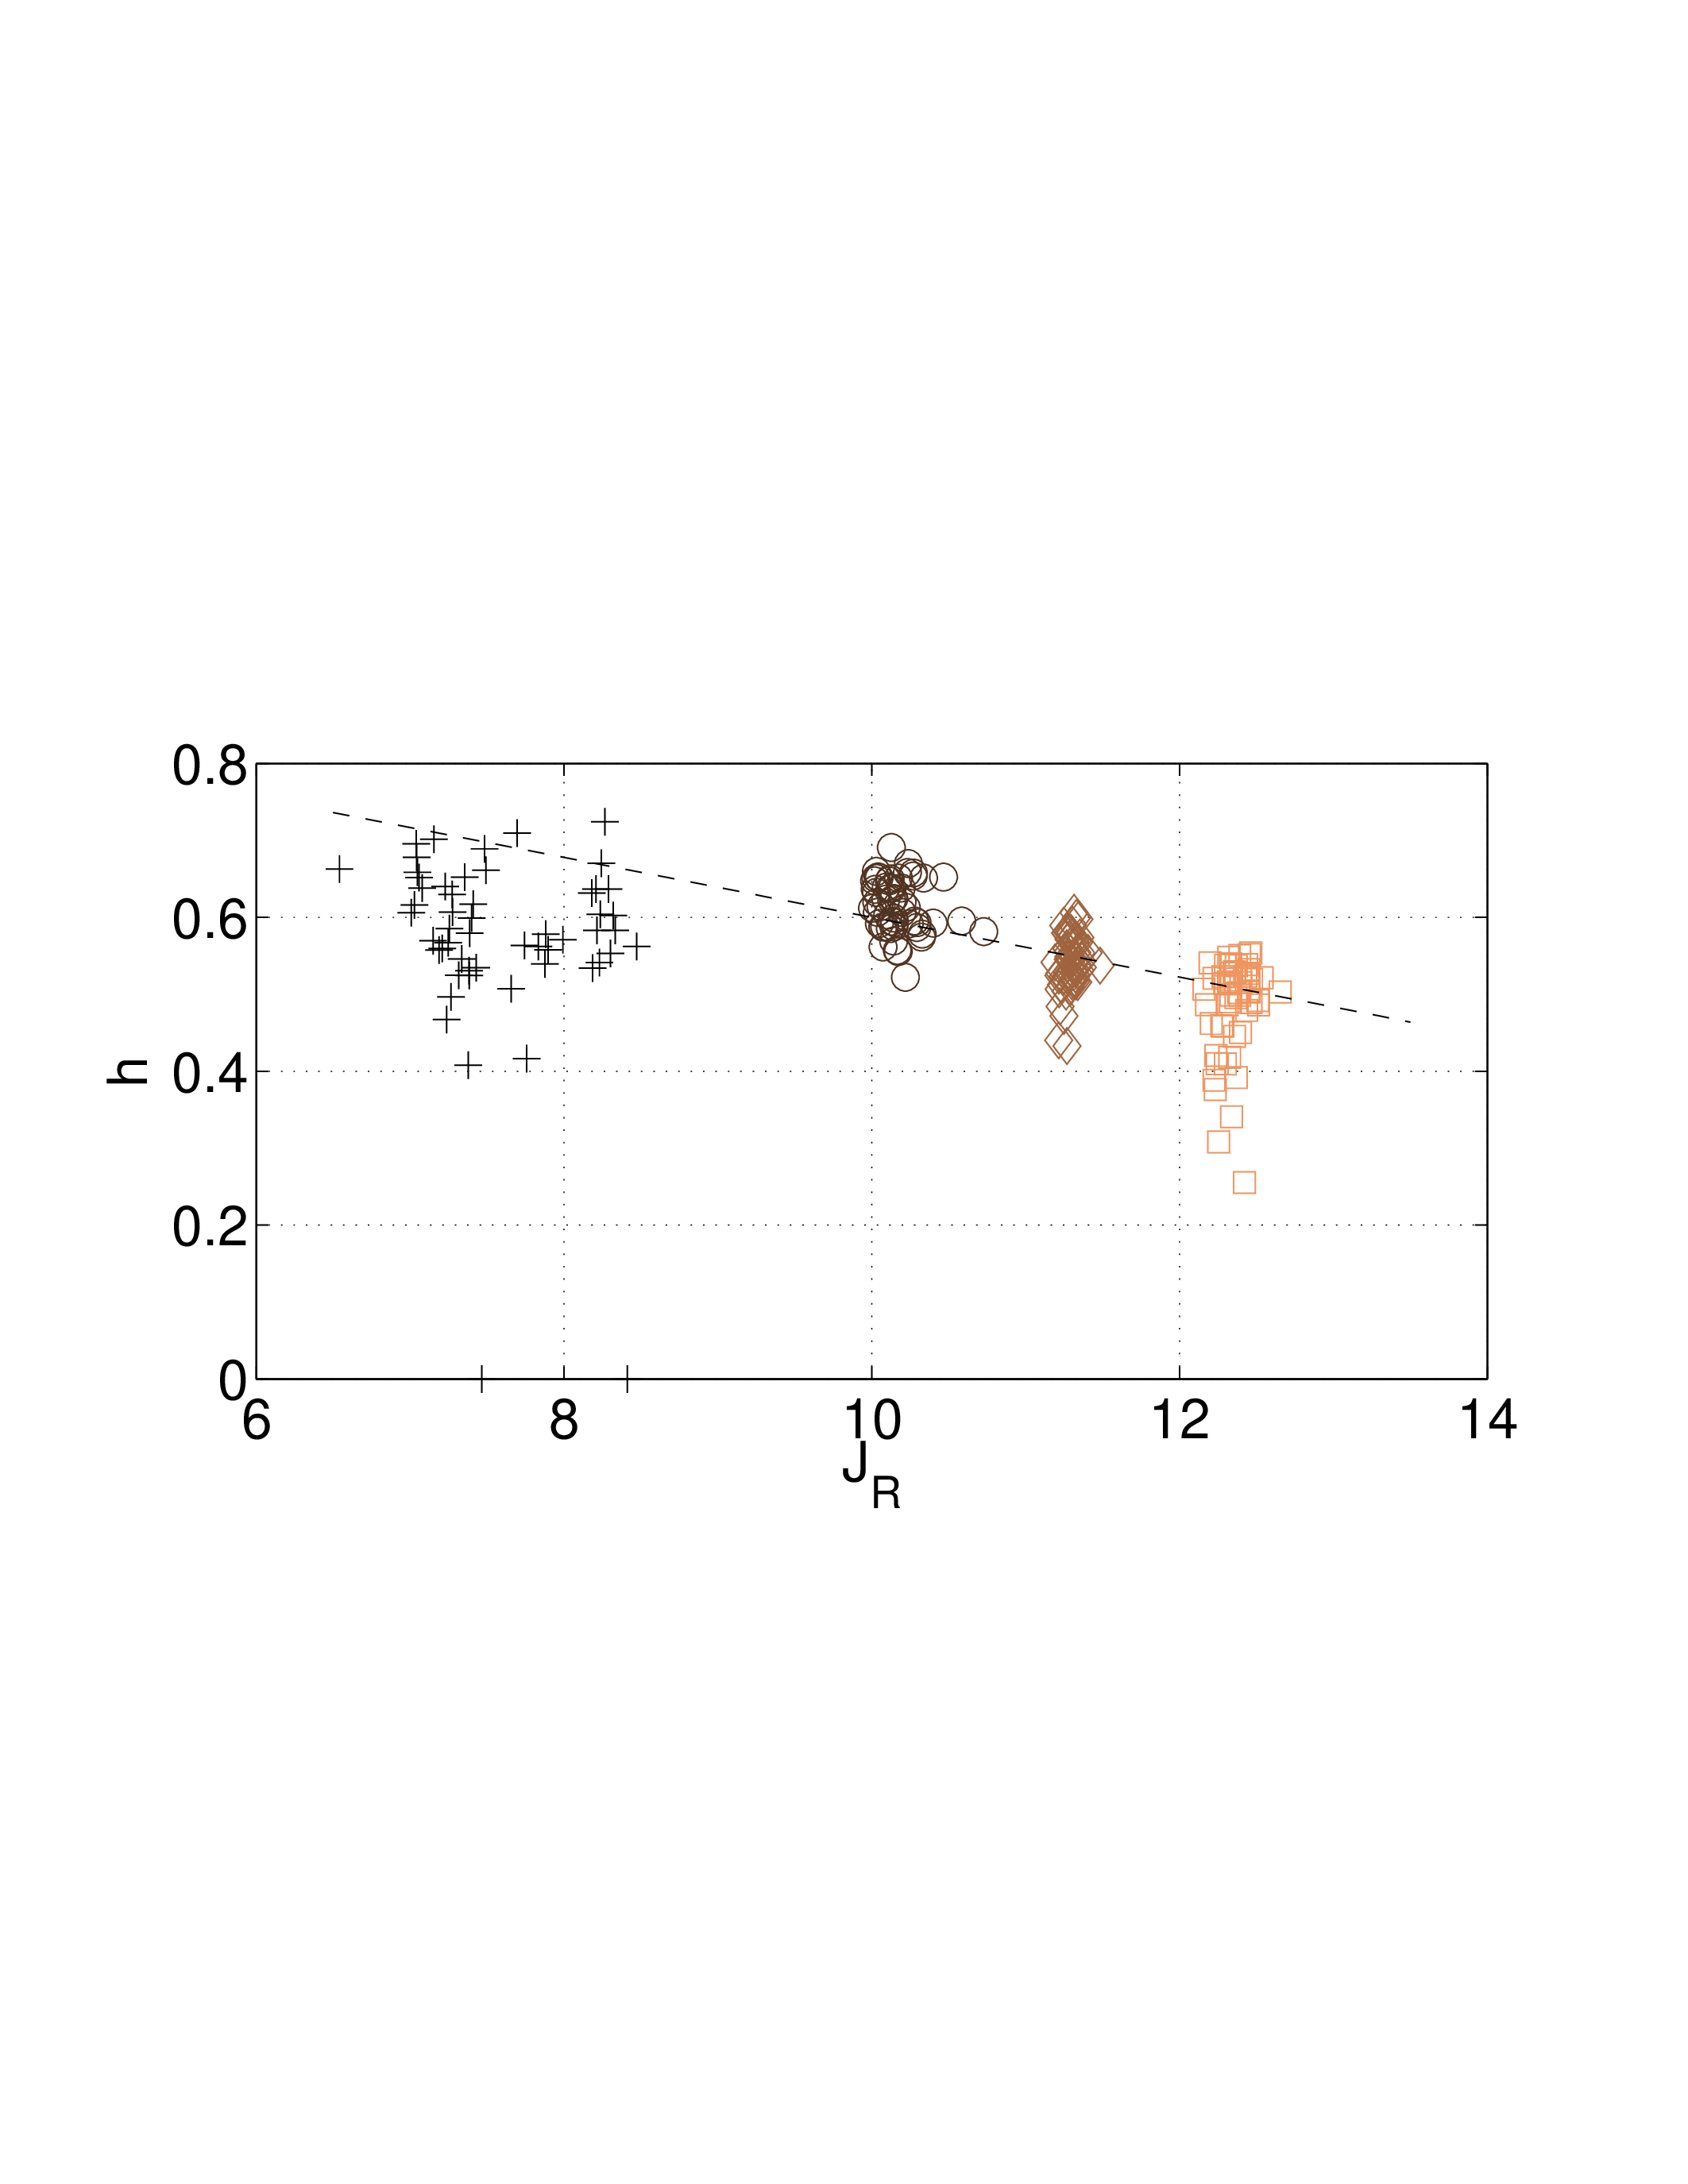}
}
\end{figure*}

\begin{figure*}
\centerline{
 \includegraphics[width=0.5\linewidth]{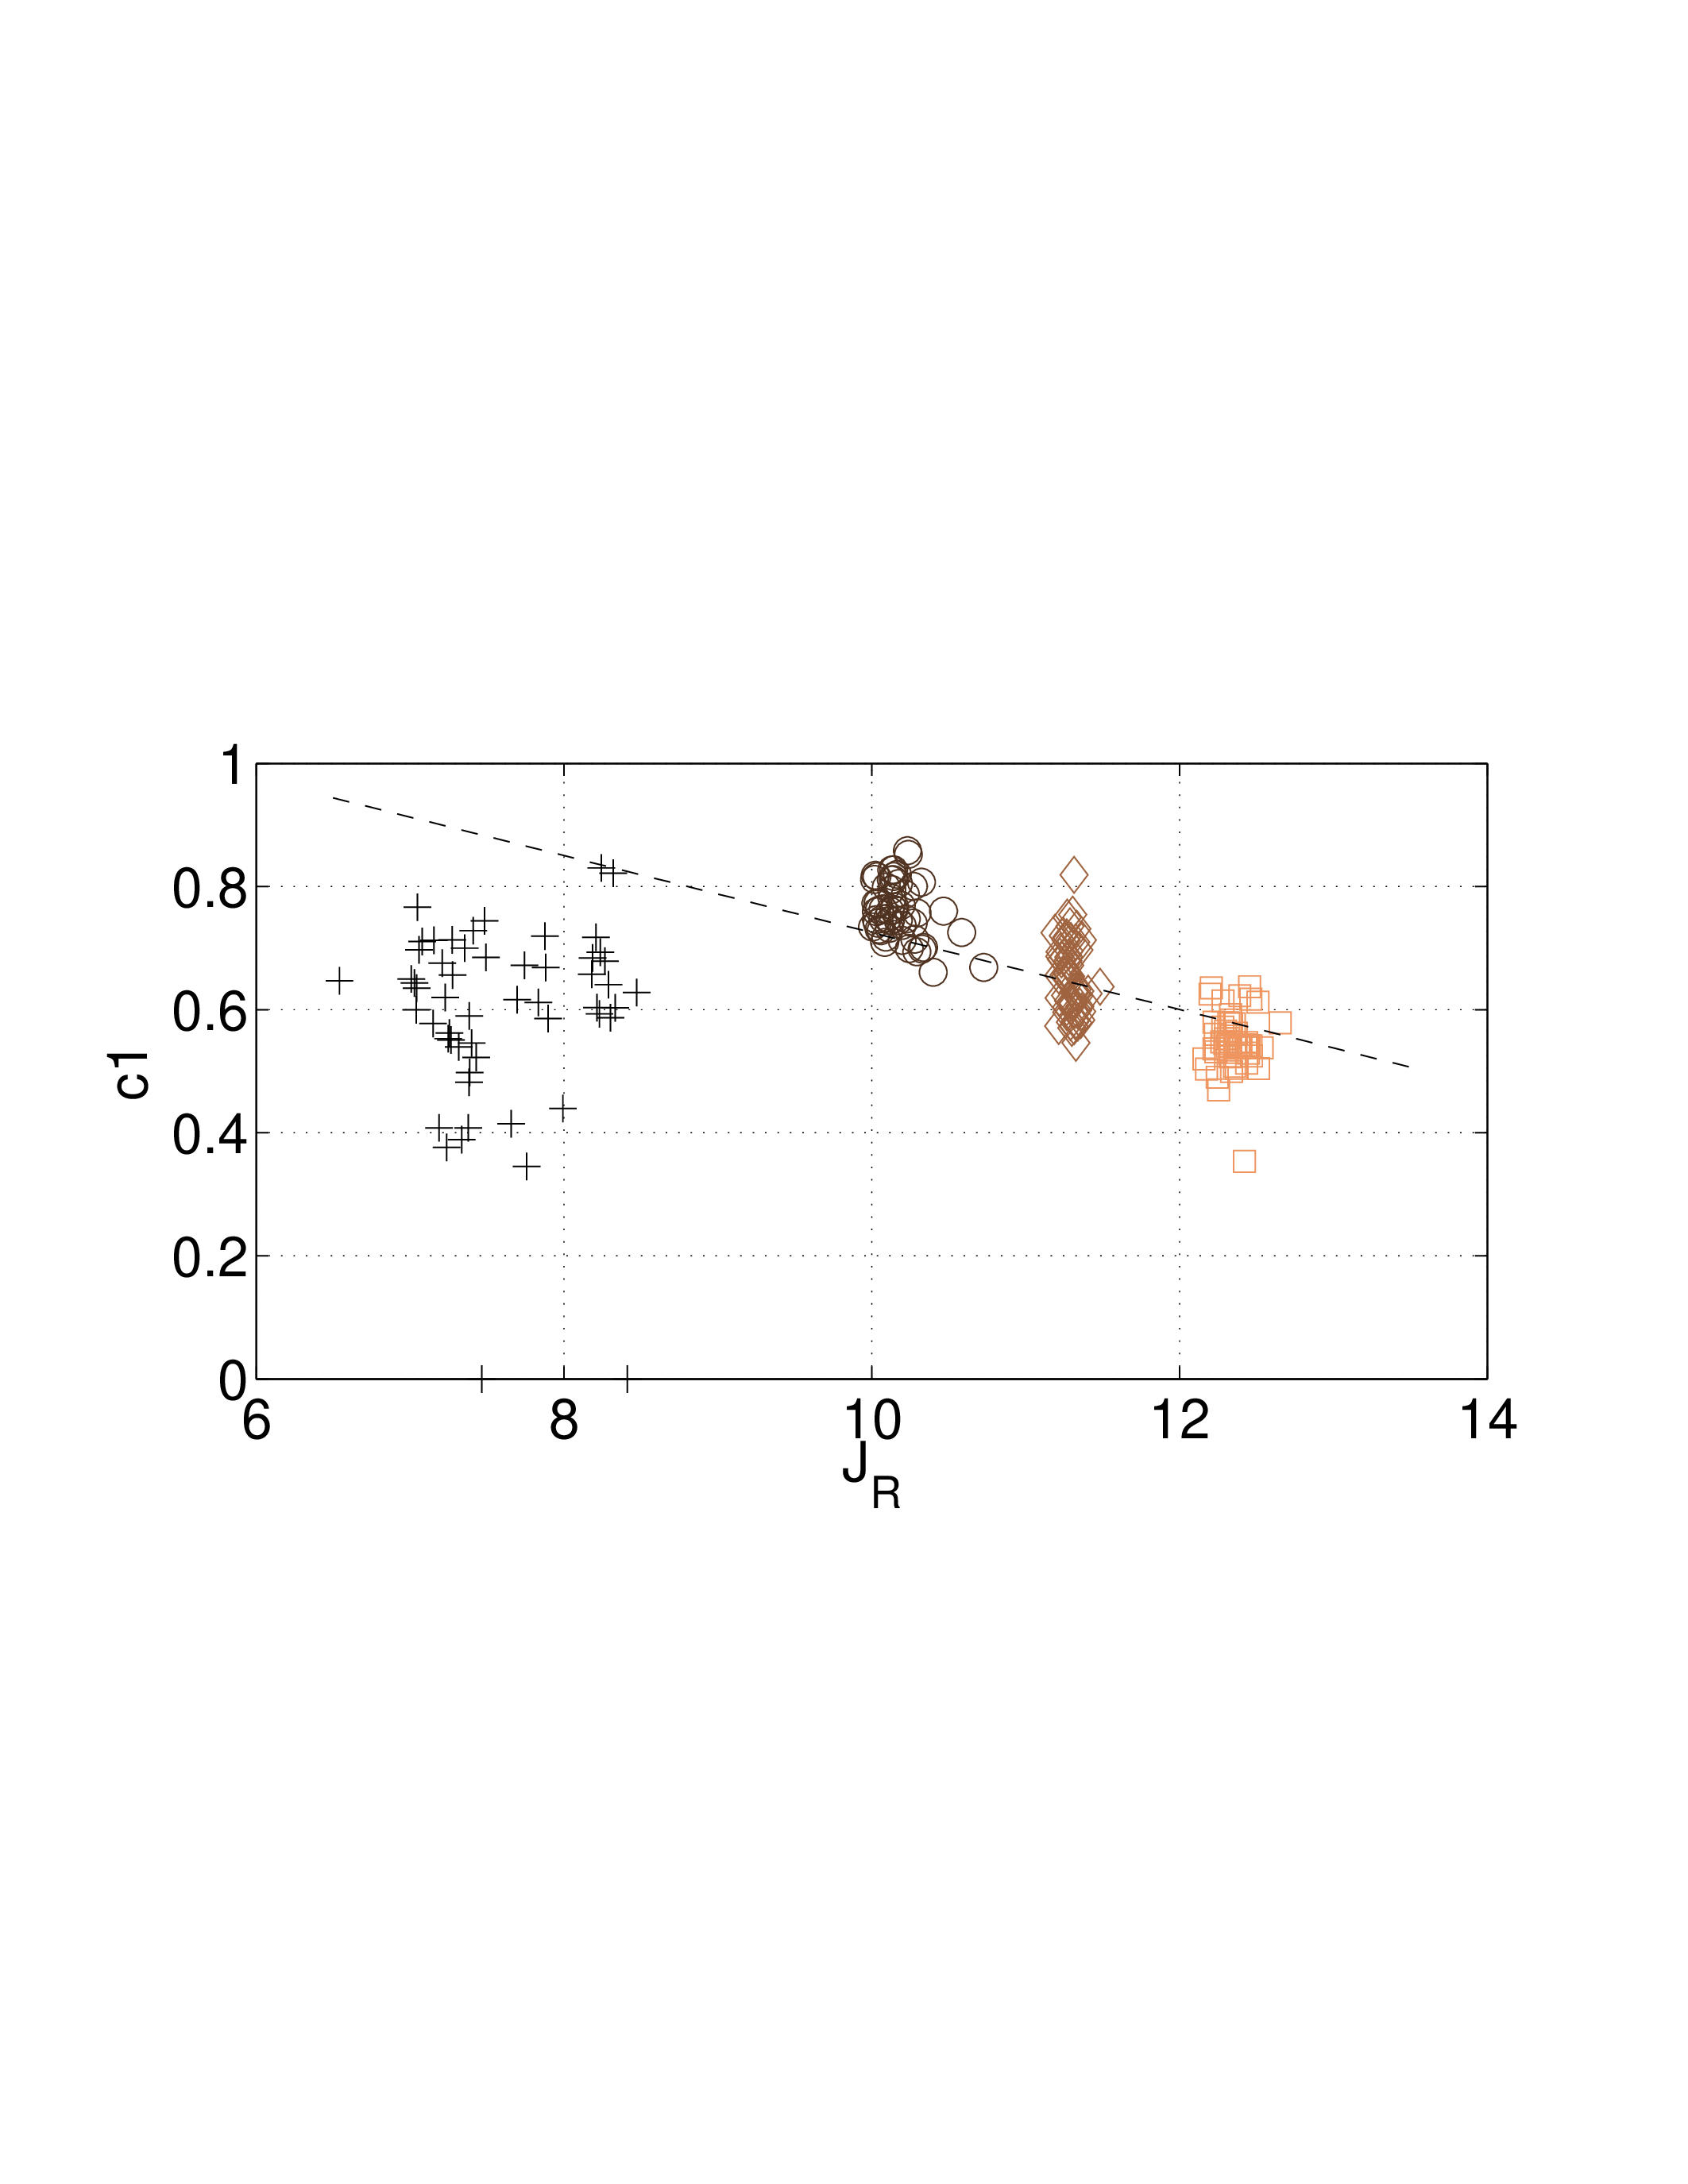}
  \includegraphics[width=0.5\linewidth]{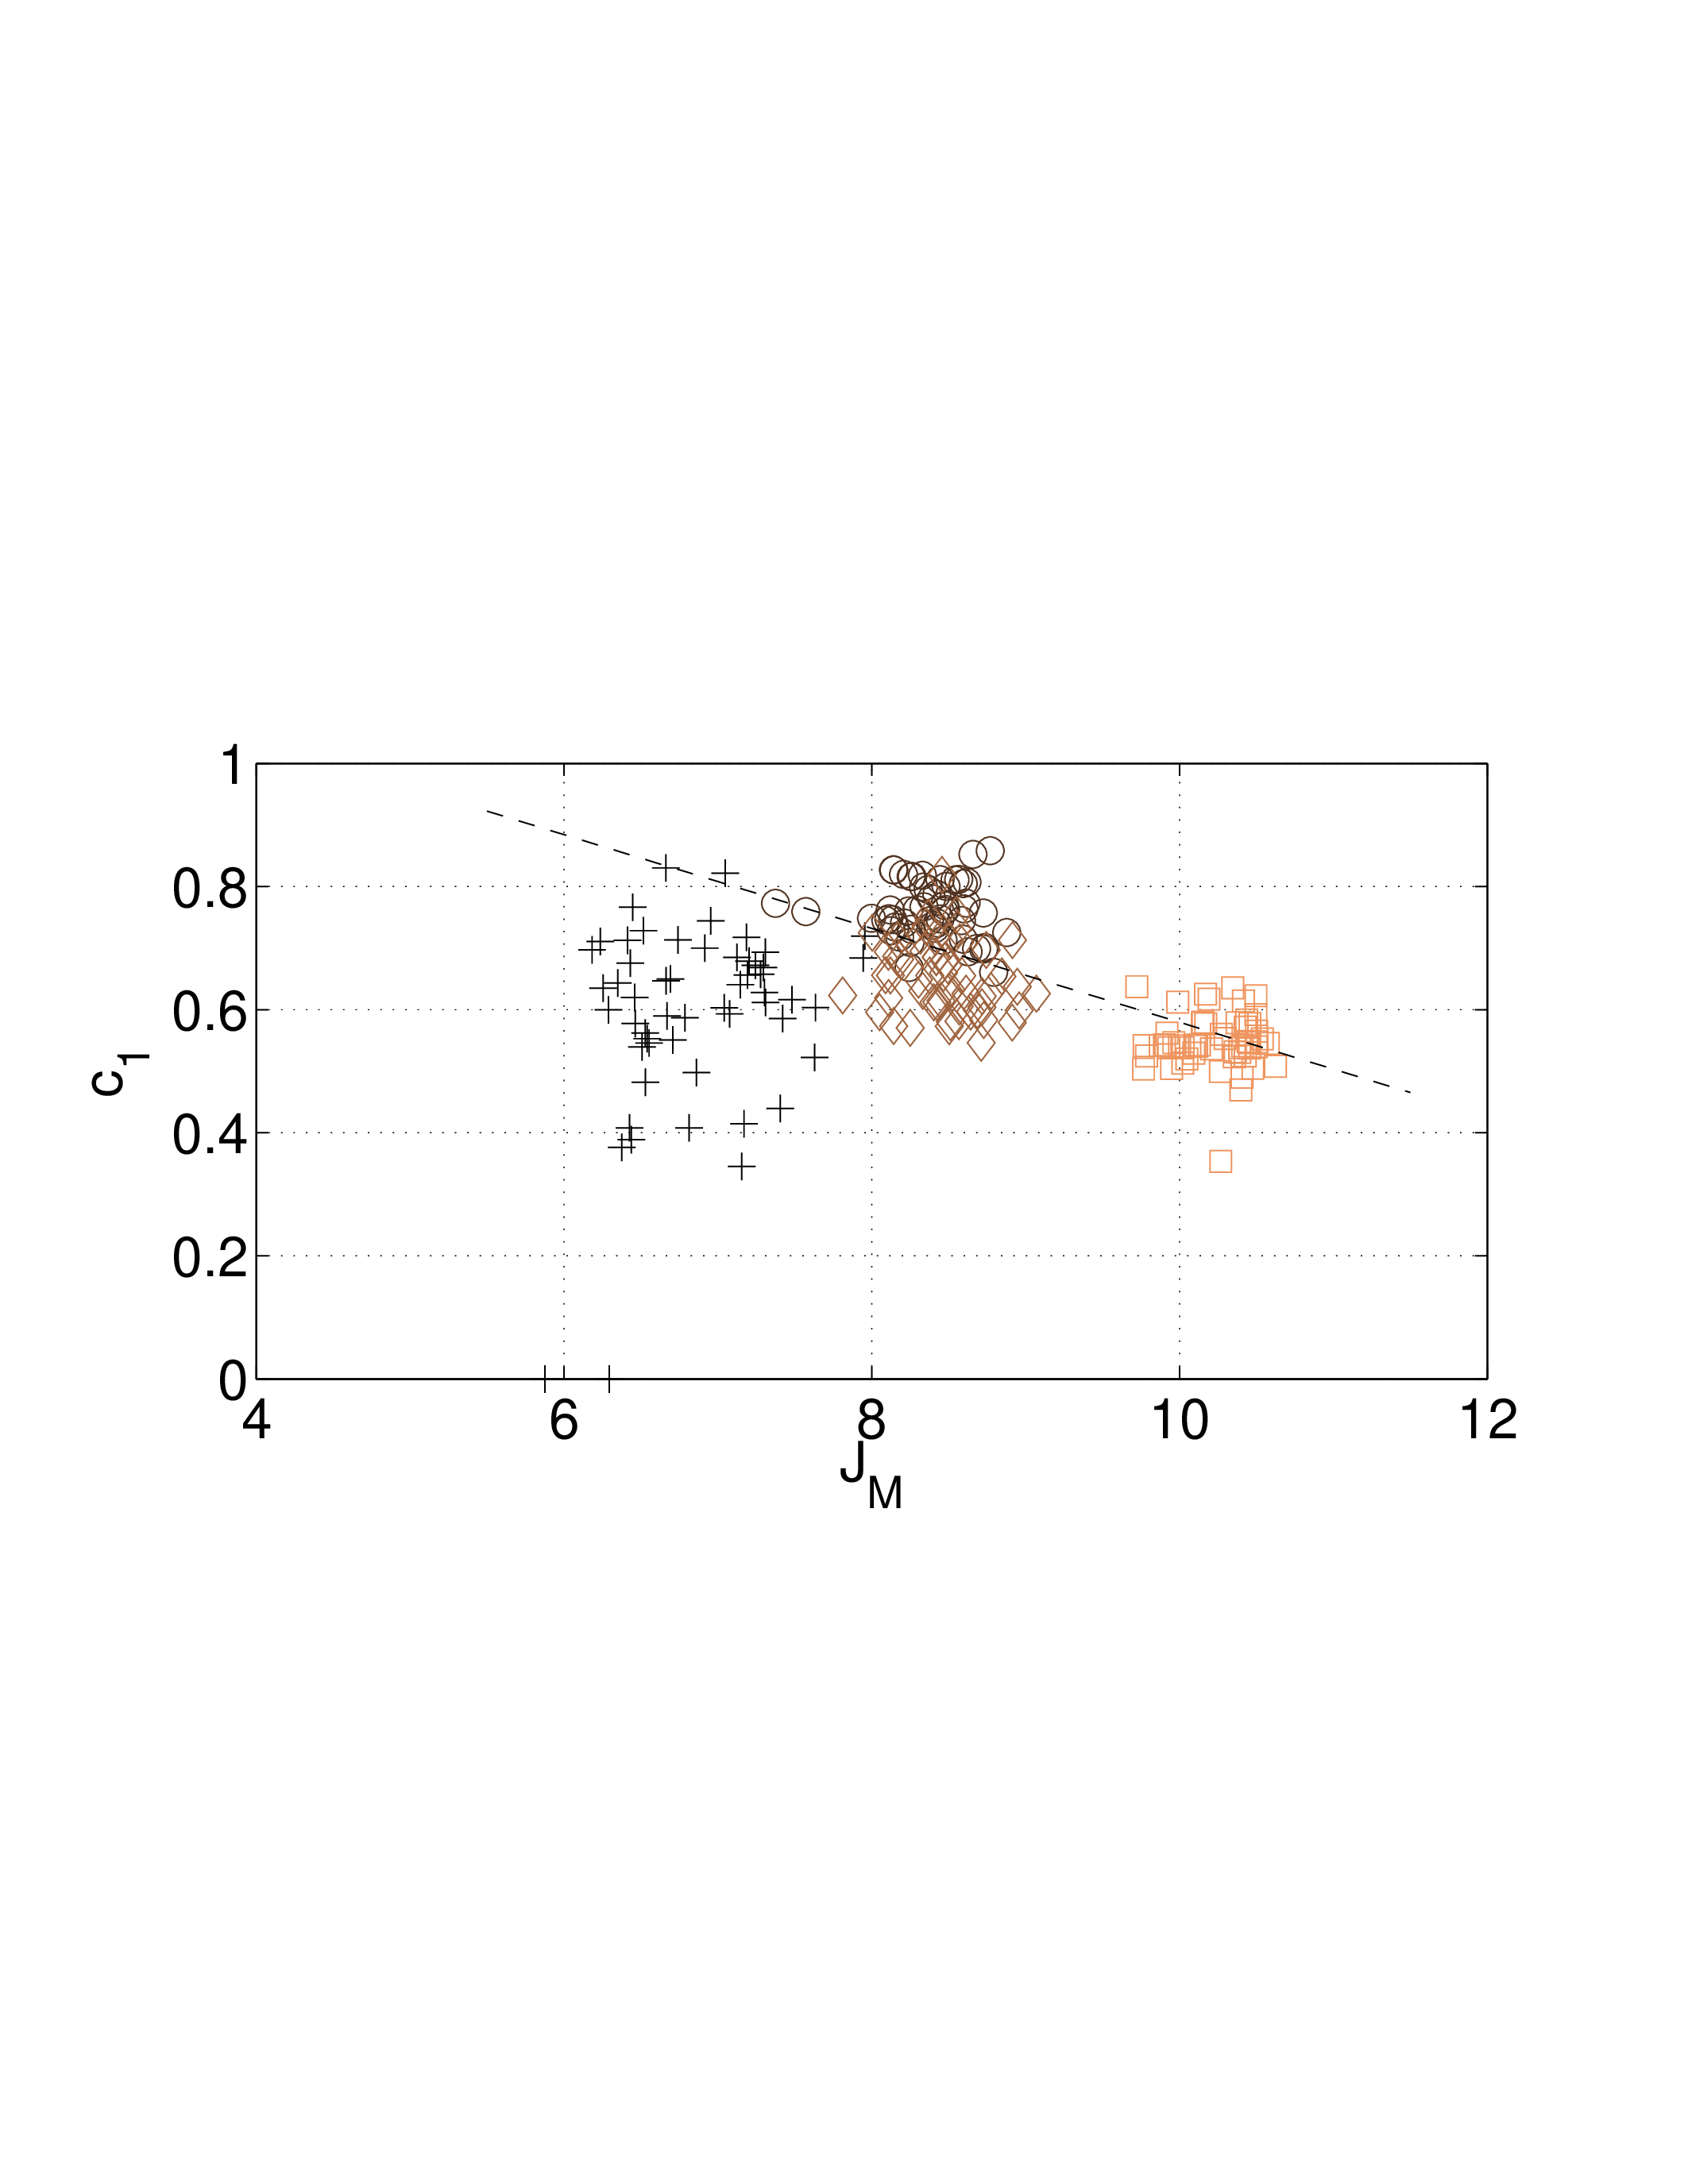}
}
\centerline{
 \includegraphics[width=0.5\linewidth]{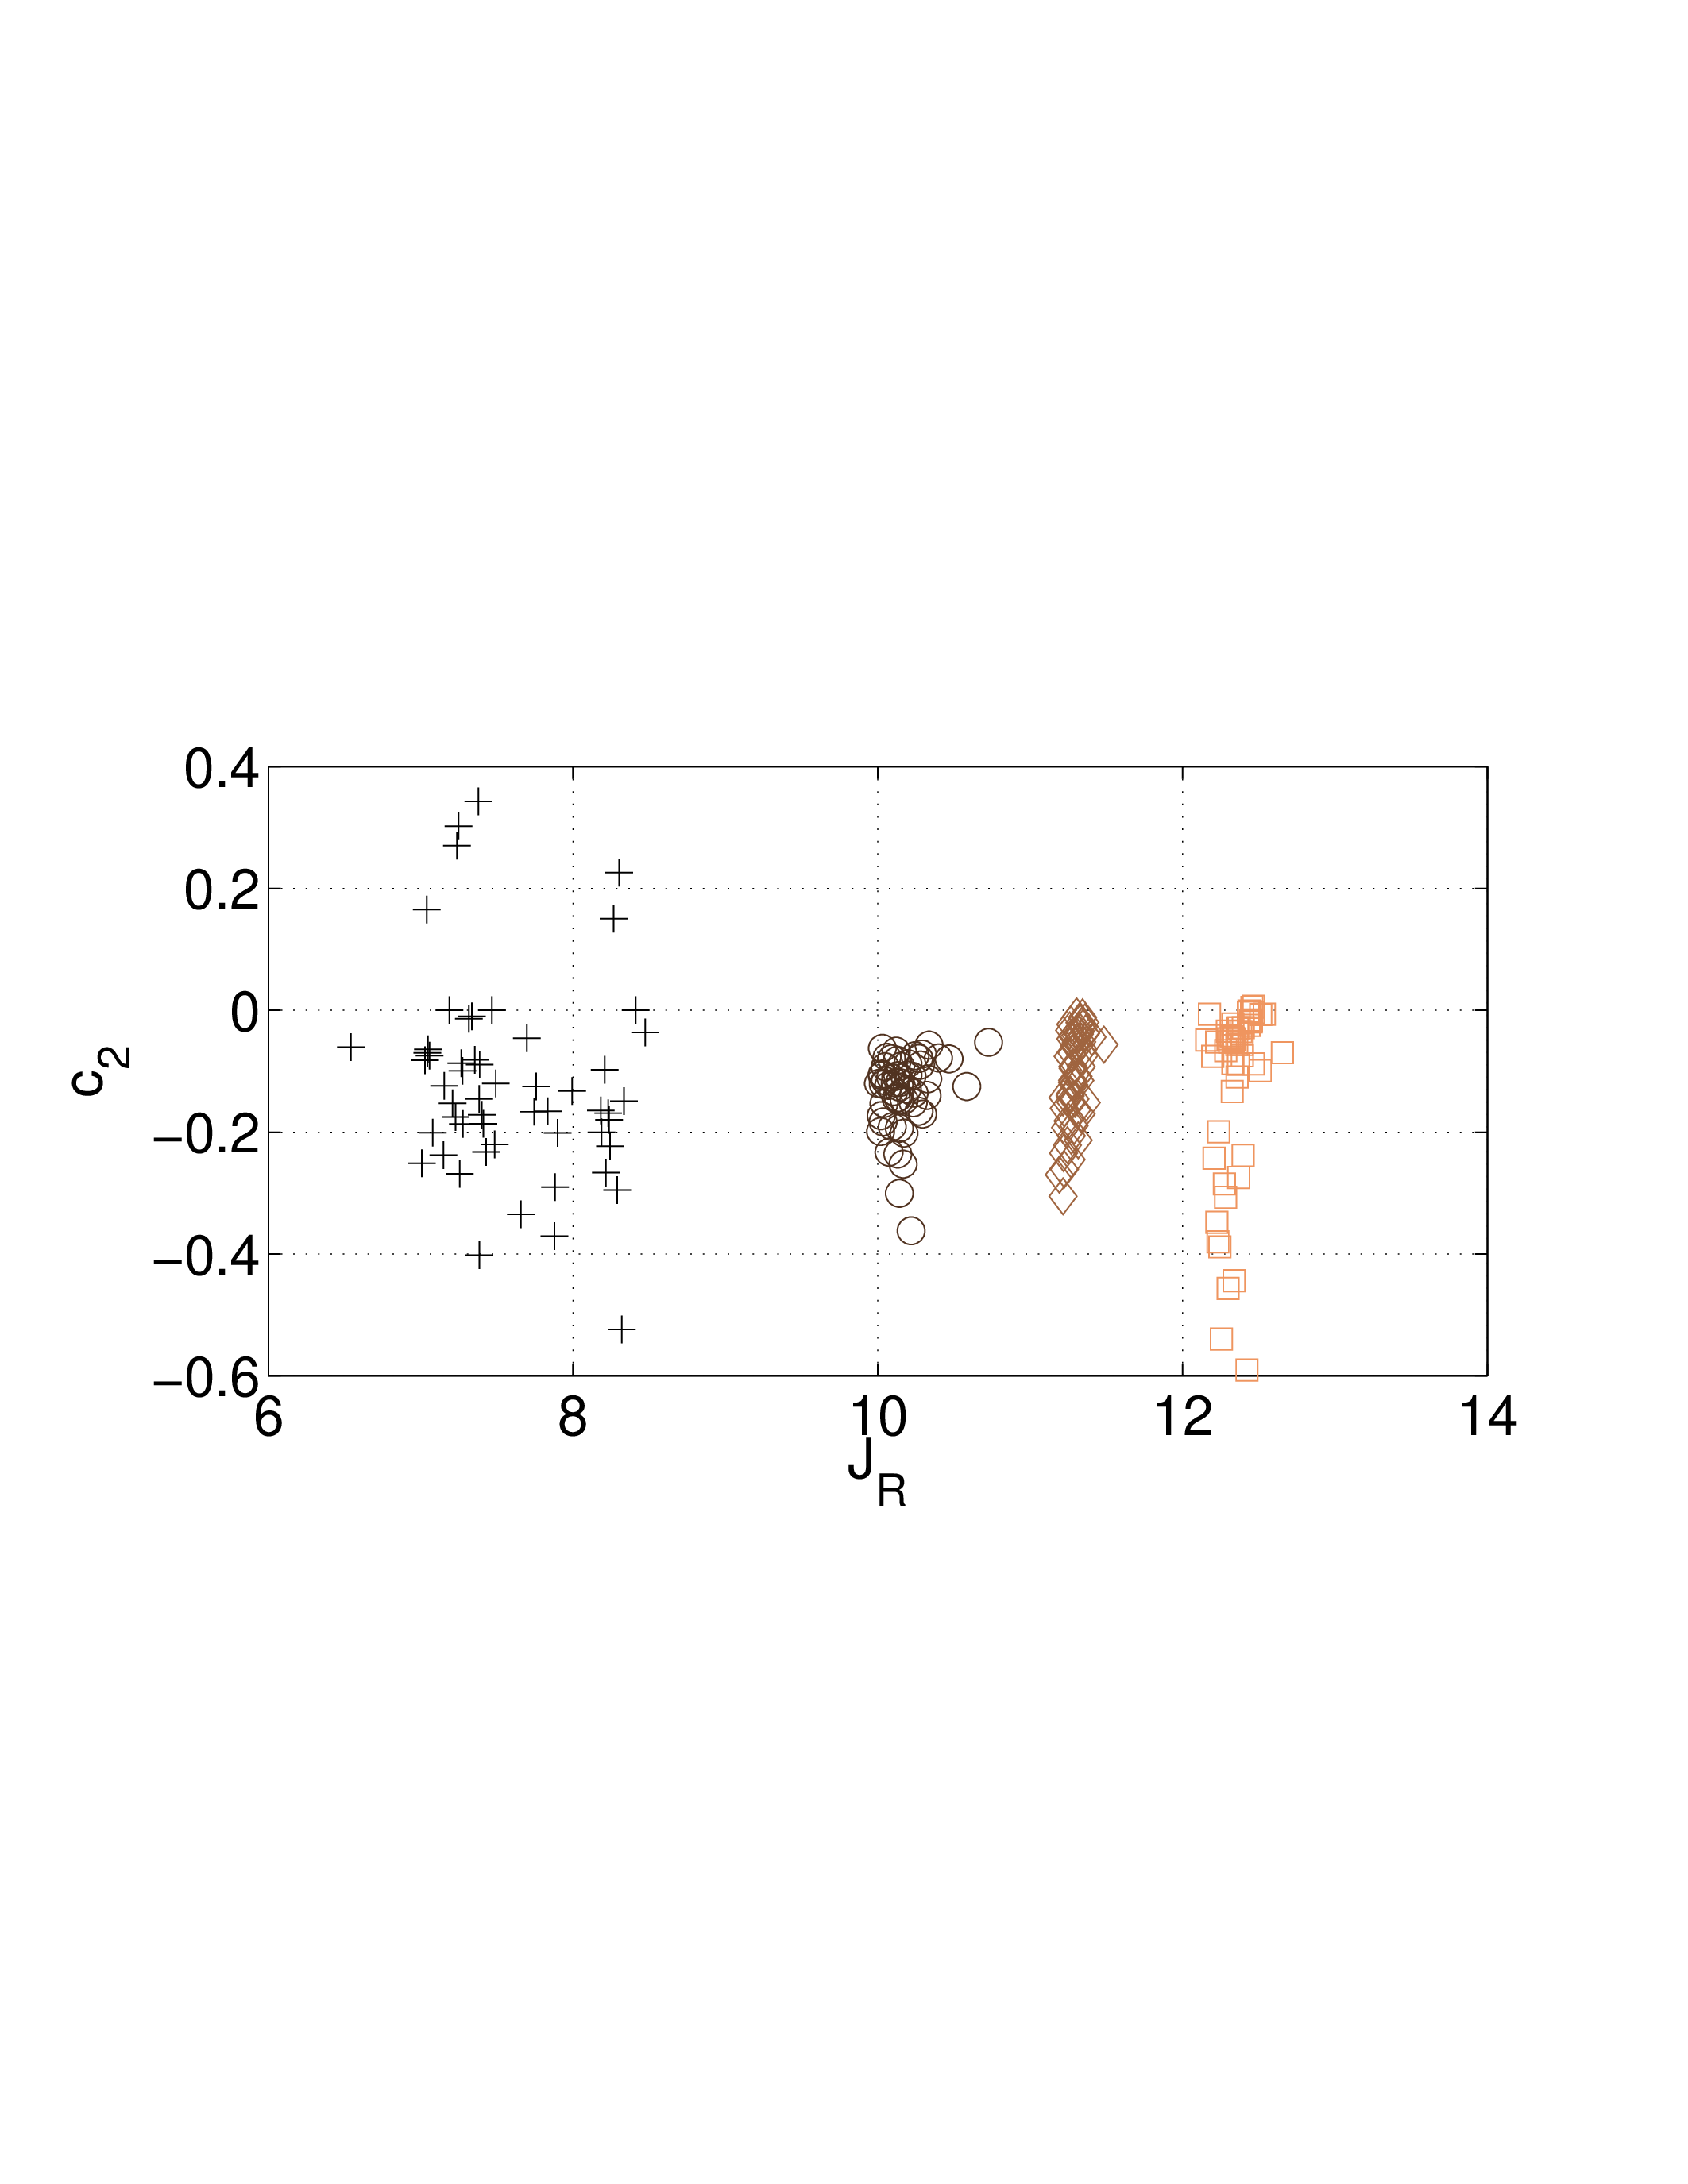}
  \includegraphics[width=0.5\linewidth]{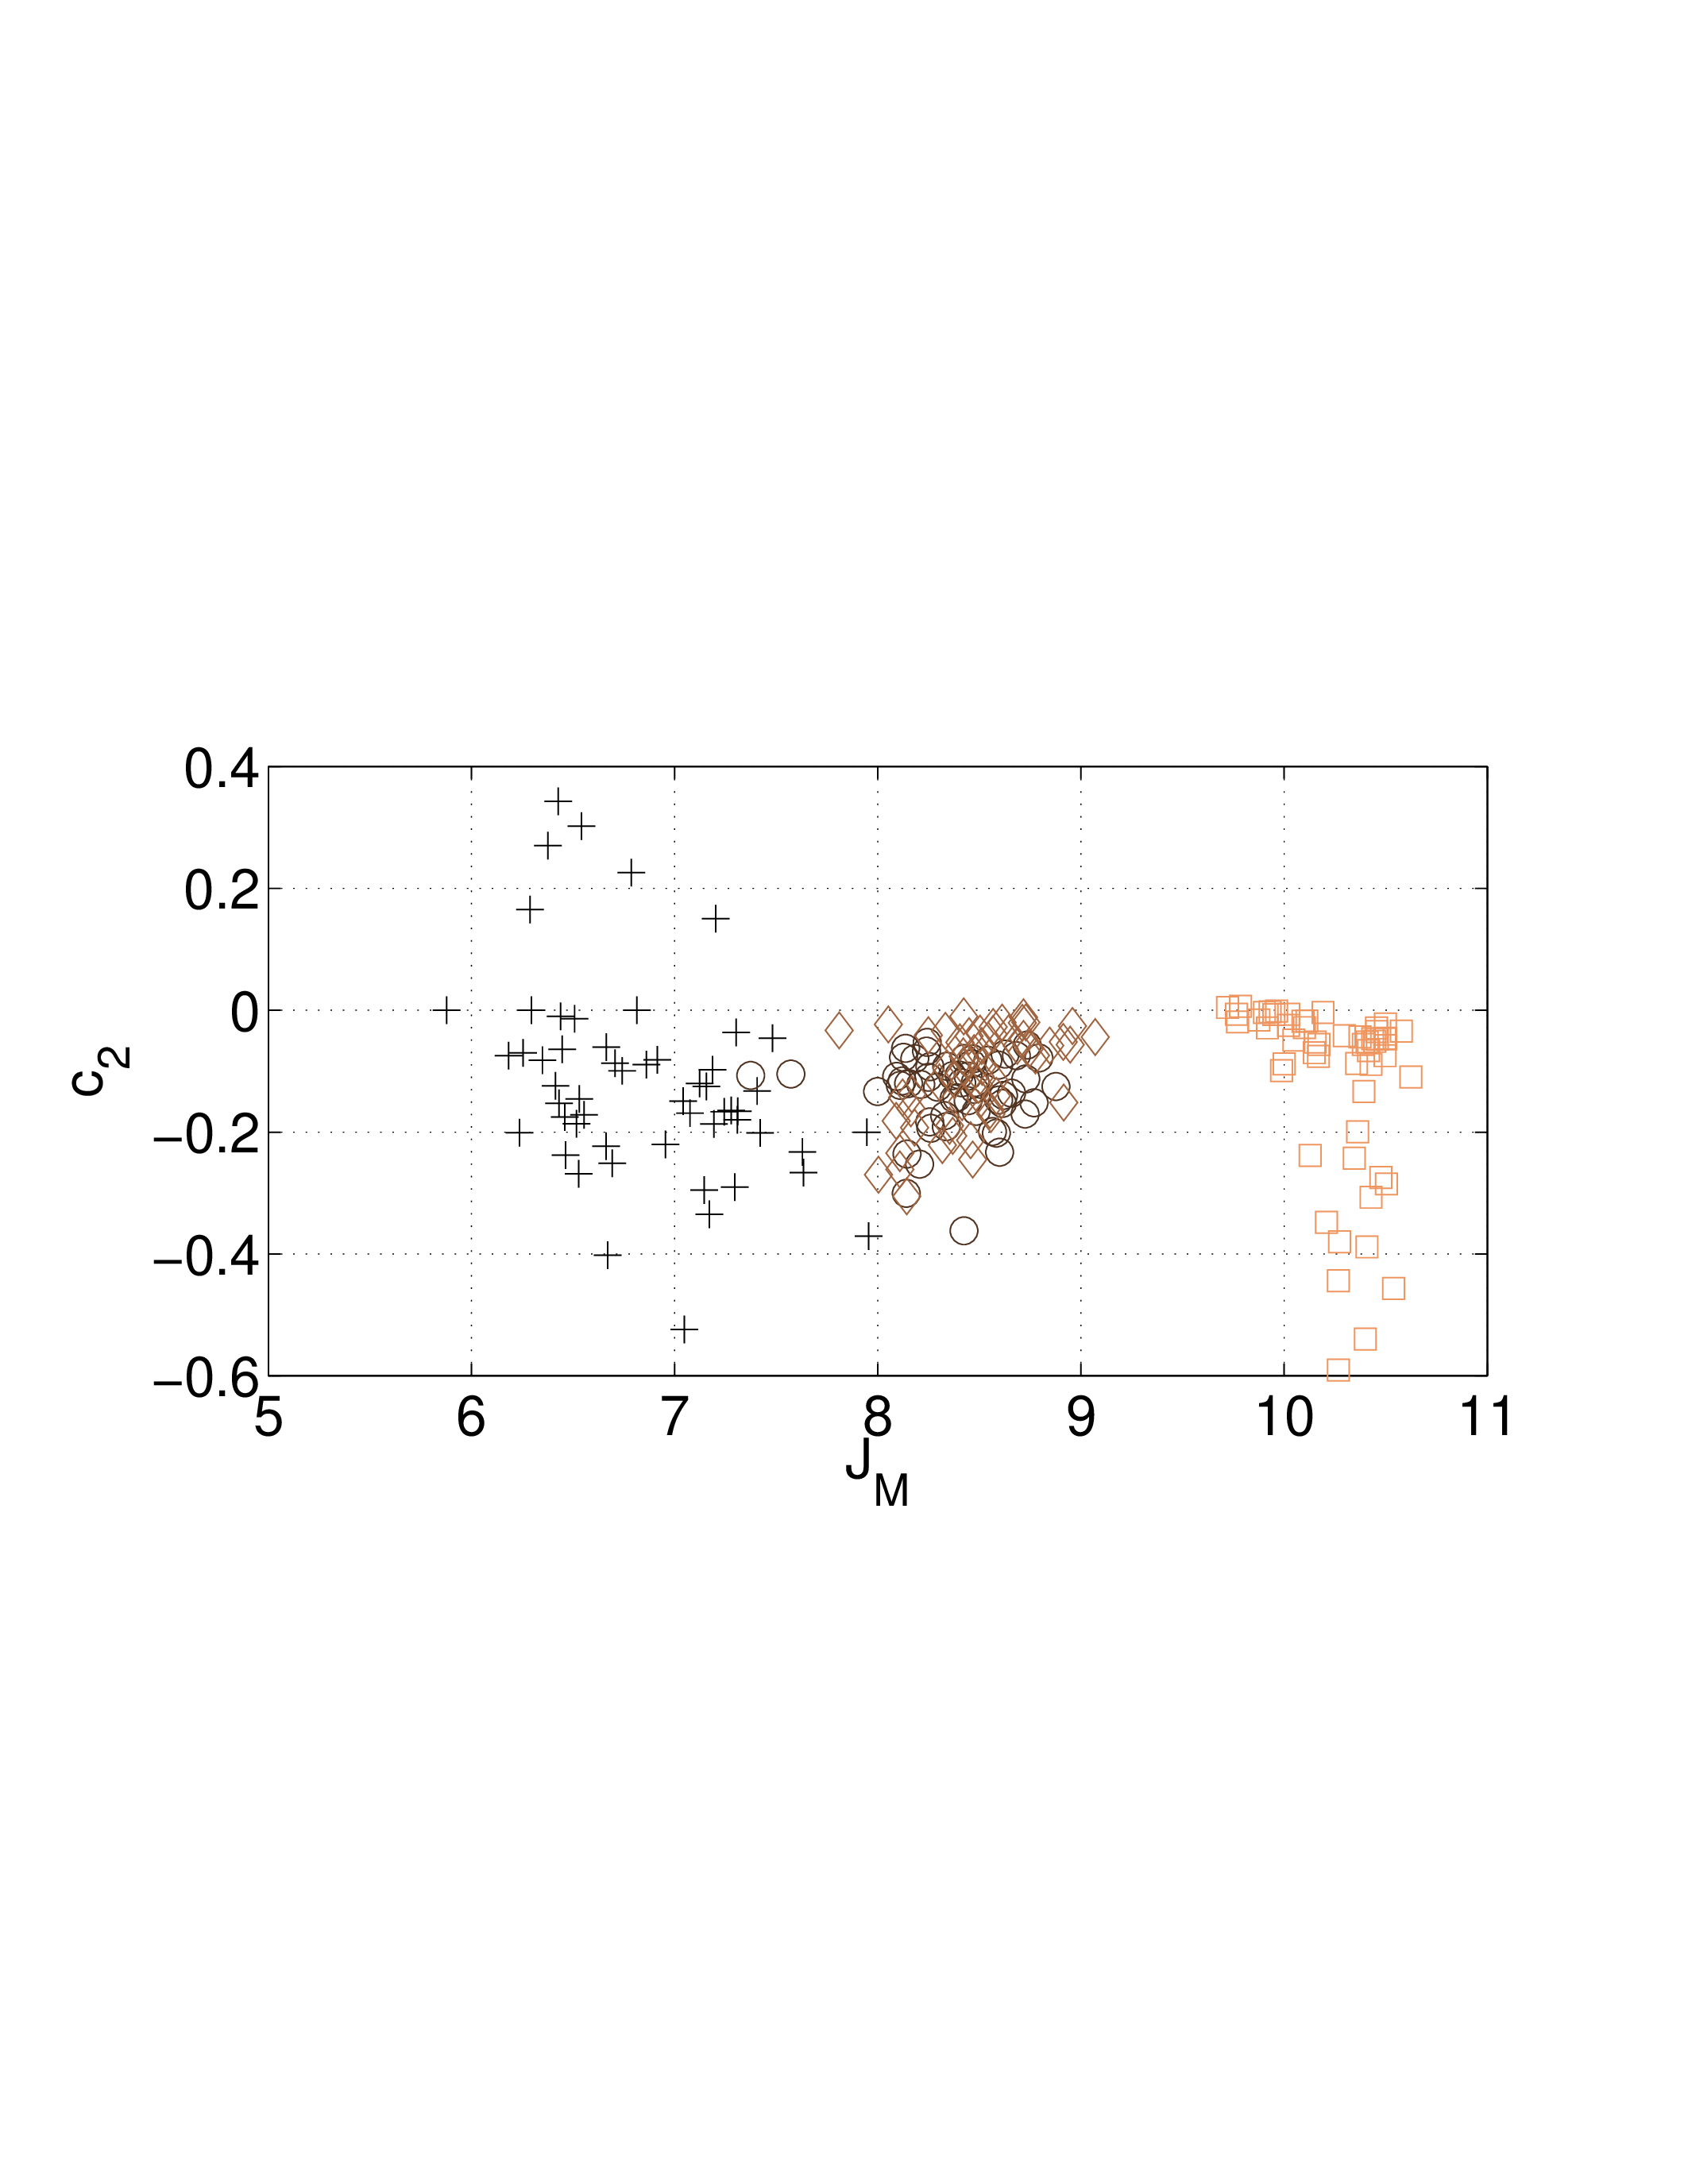}
}
\end{figure*}

\begin{figure*}
\centerline{
 \includegraphics[width=.33\textwidth]{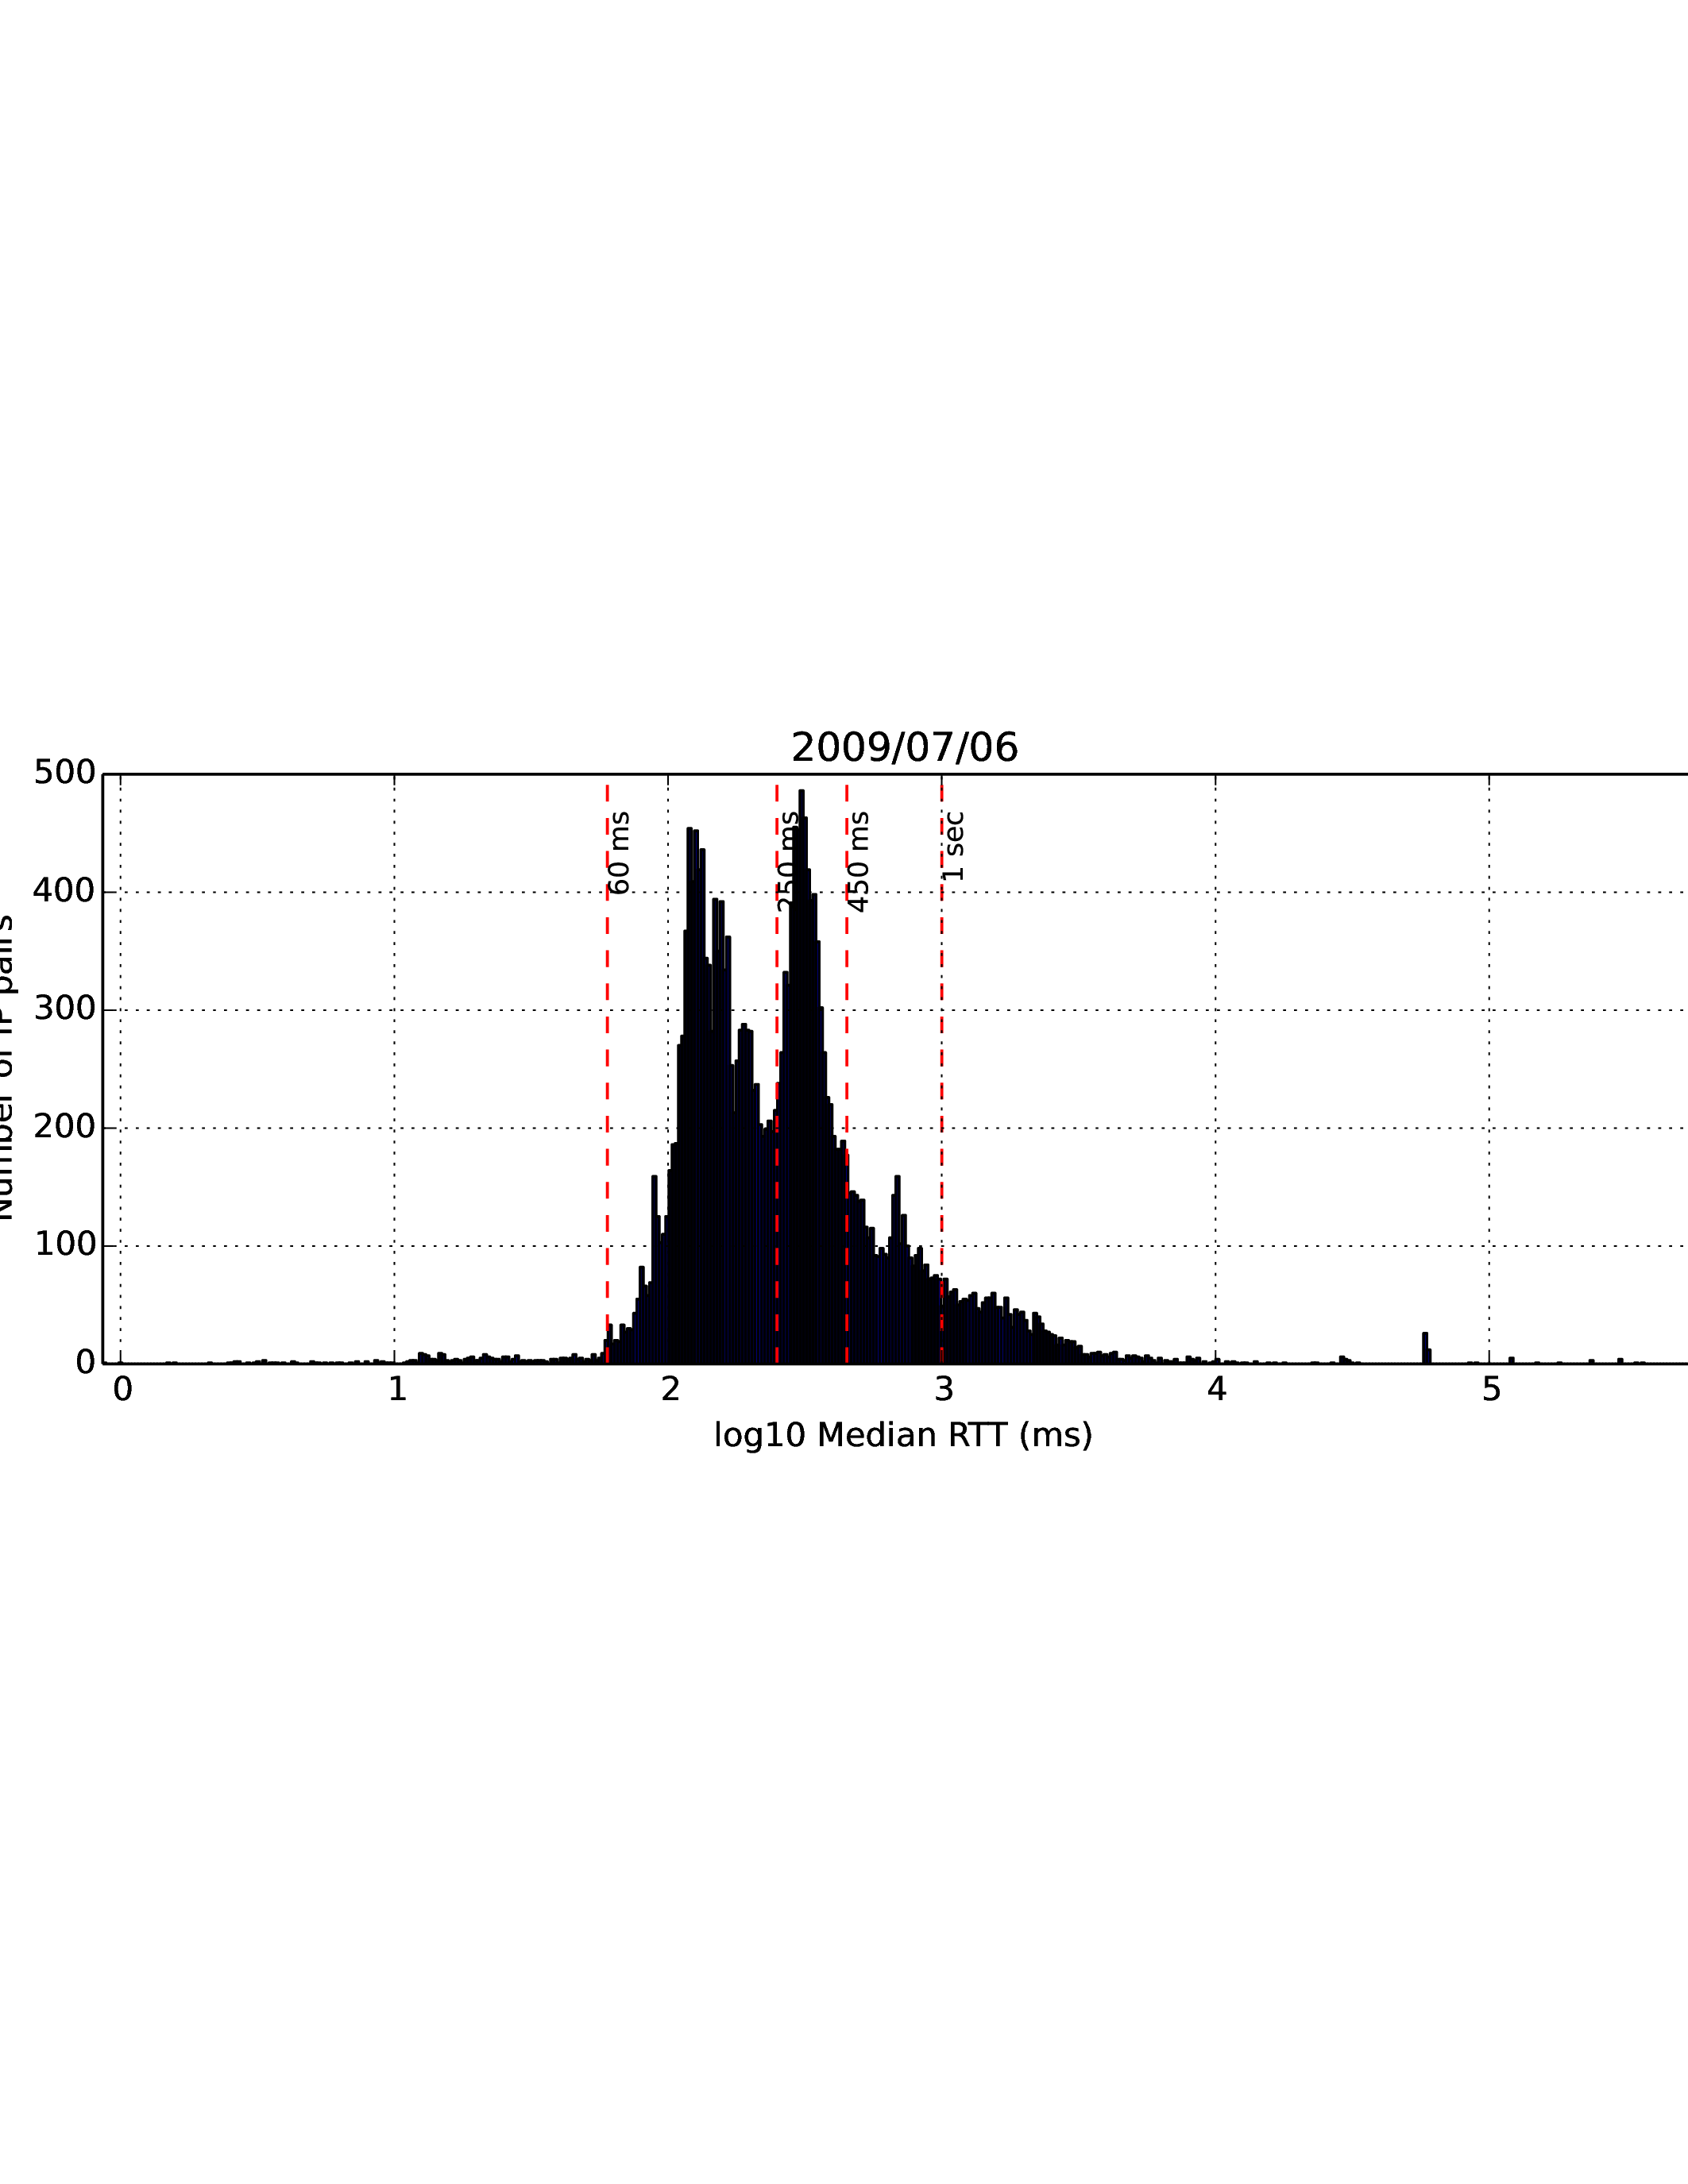}
 \includegraphics[width=.33\textwidth]{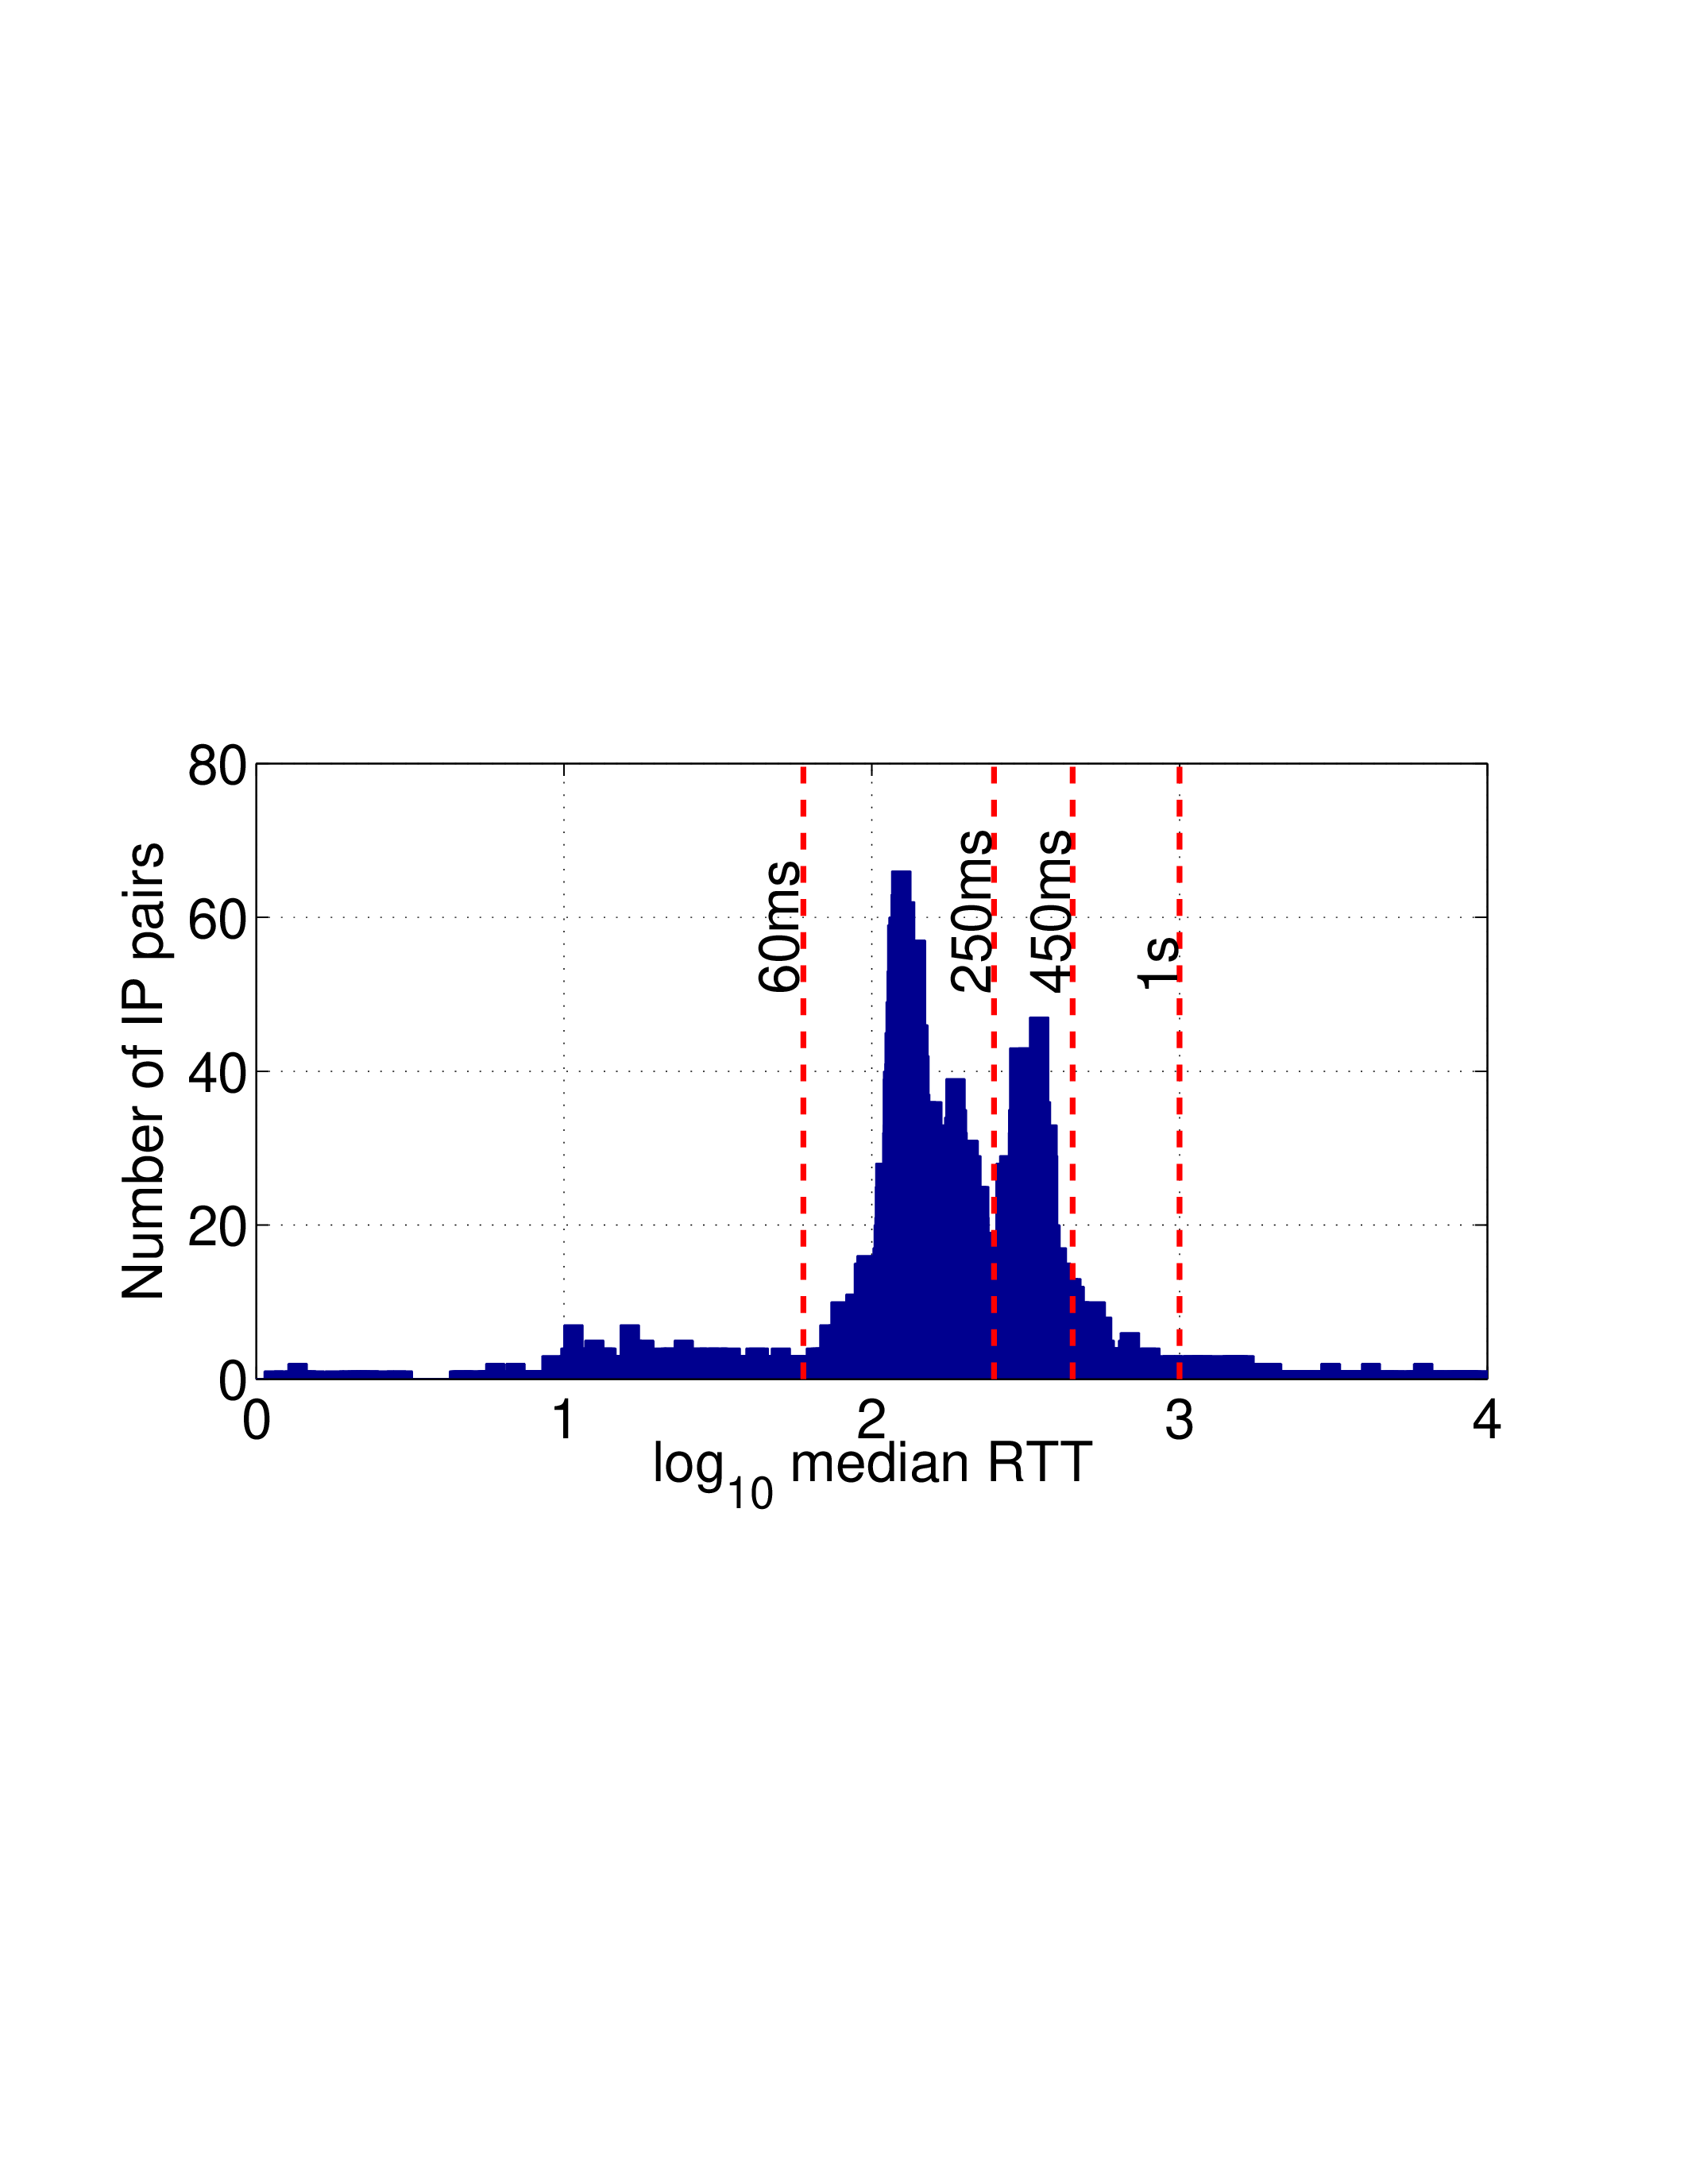}
 \includegraphics[width=.33\textwidth]{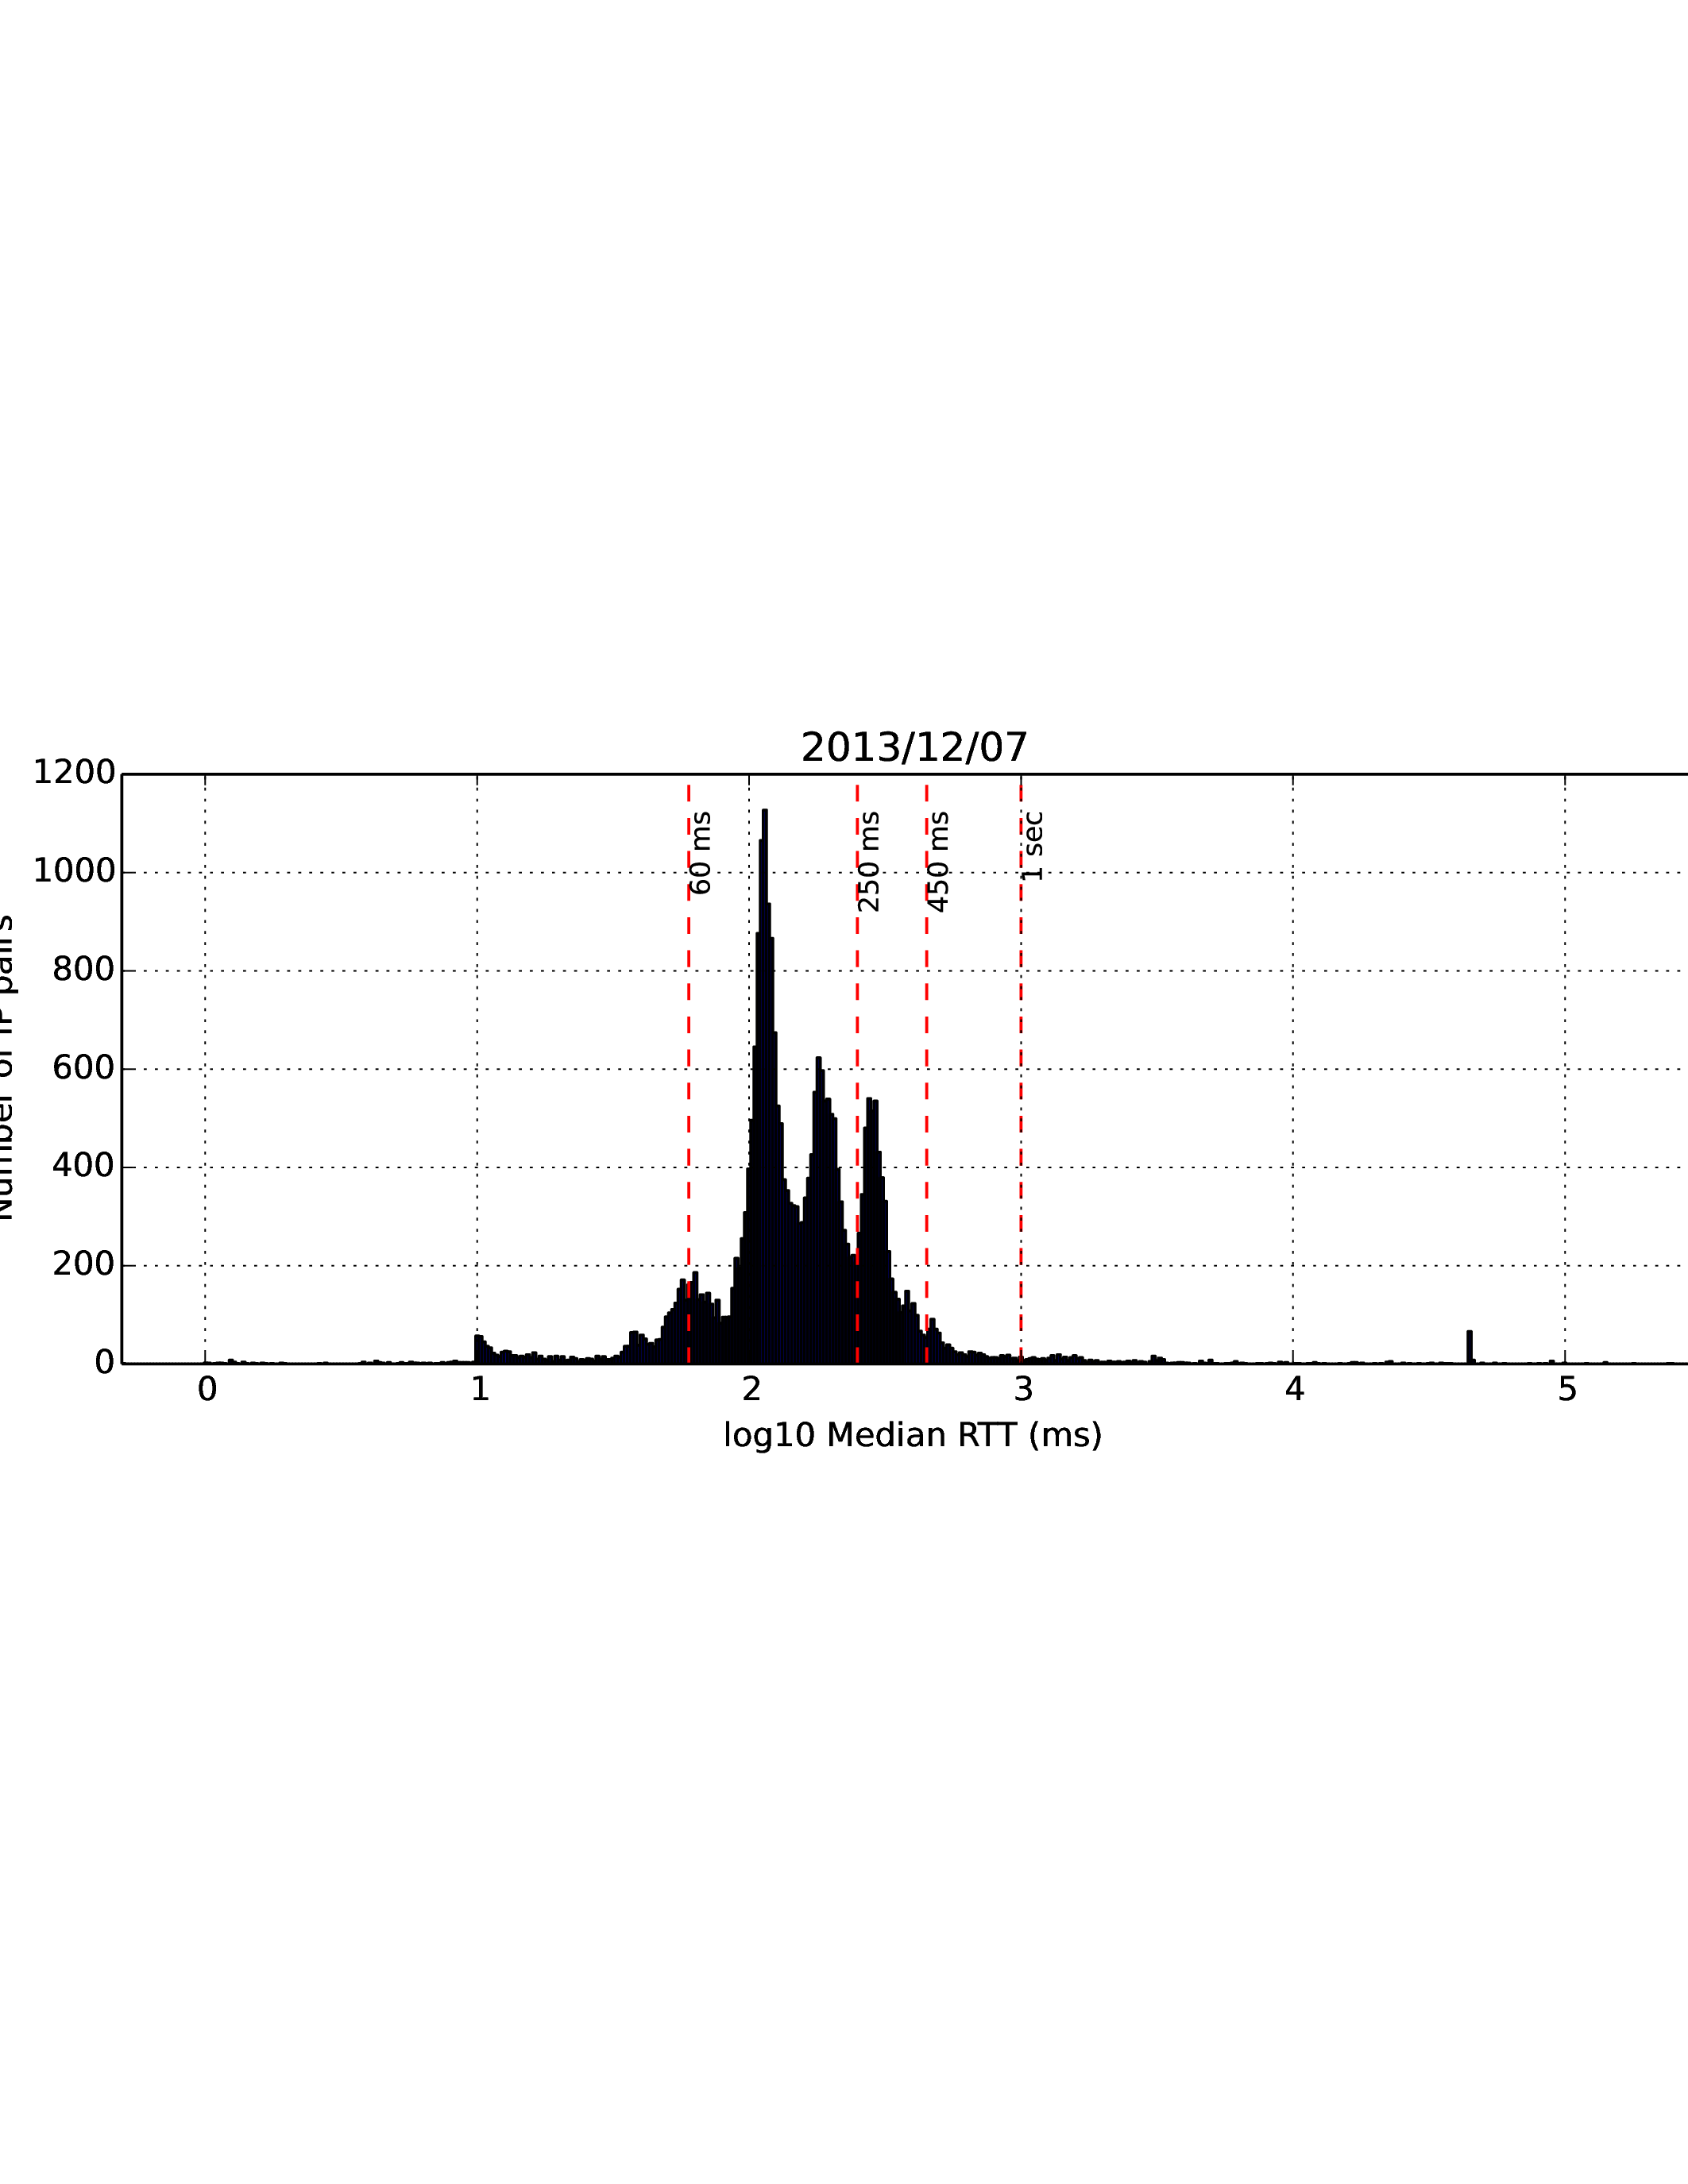}
}
\centerline{
 \includegraphics[width=.33\textwidth]{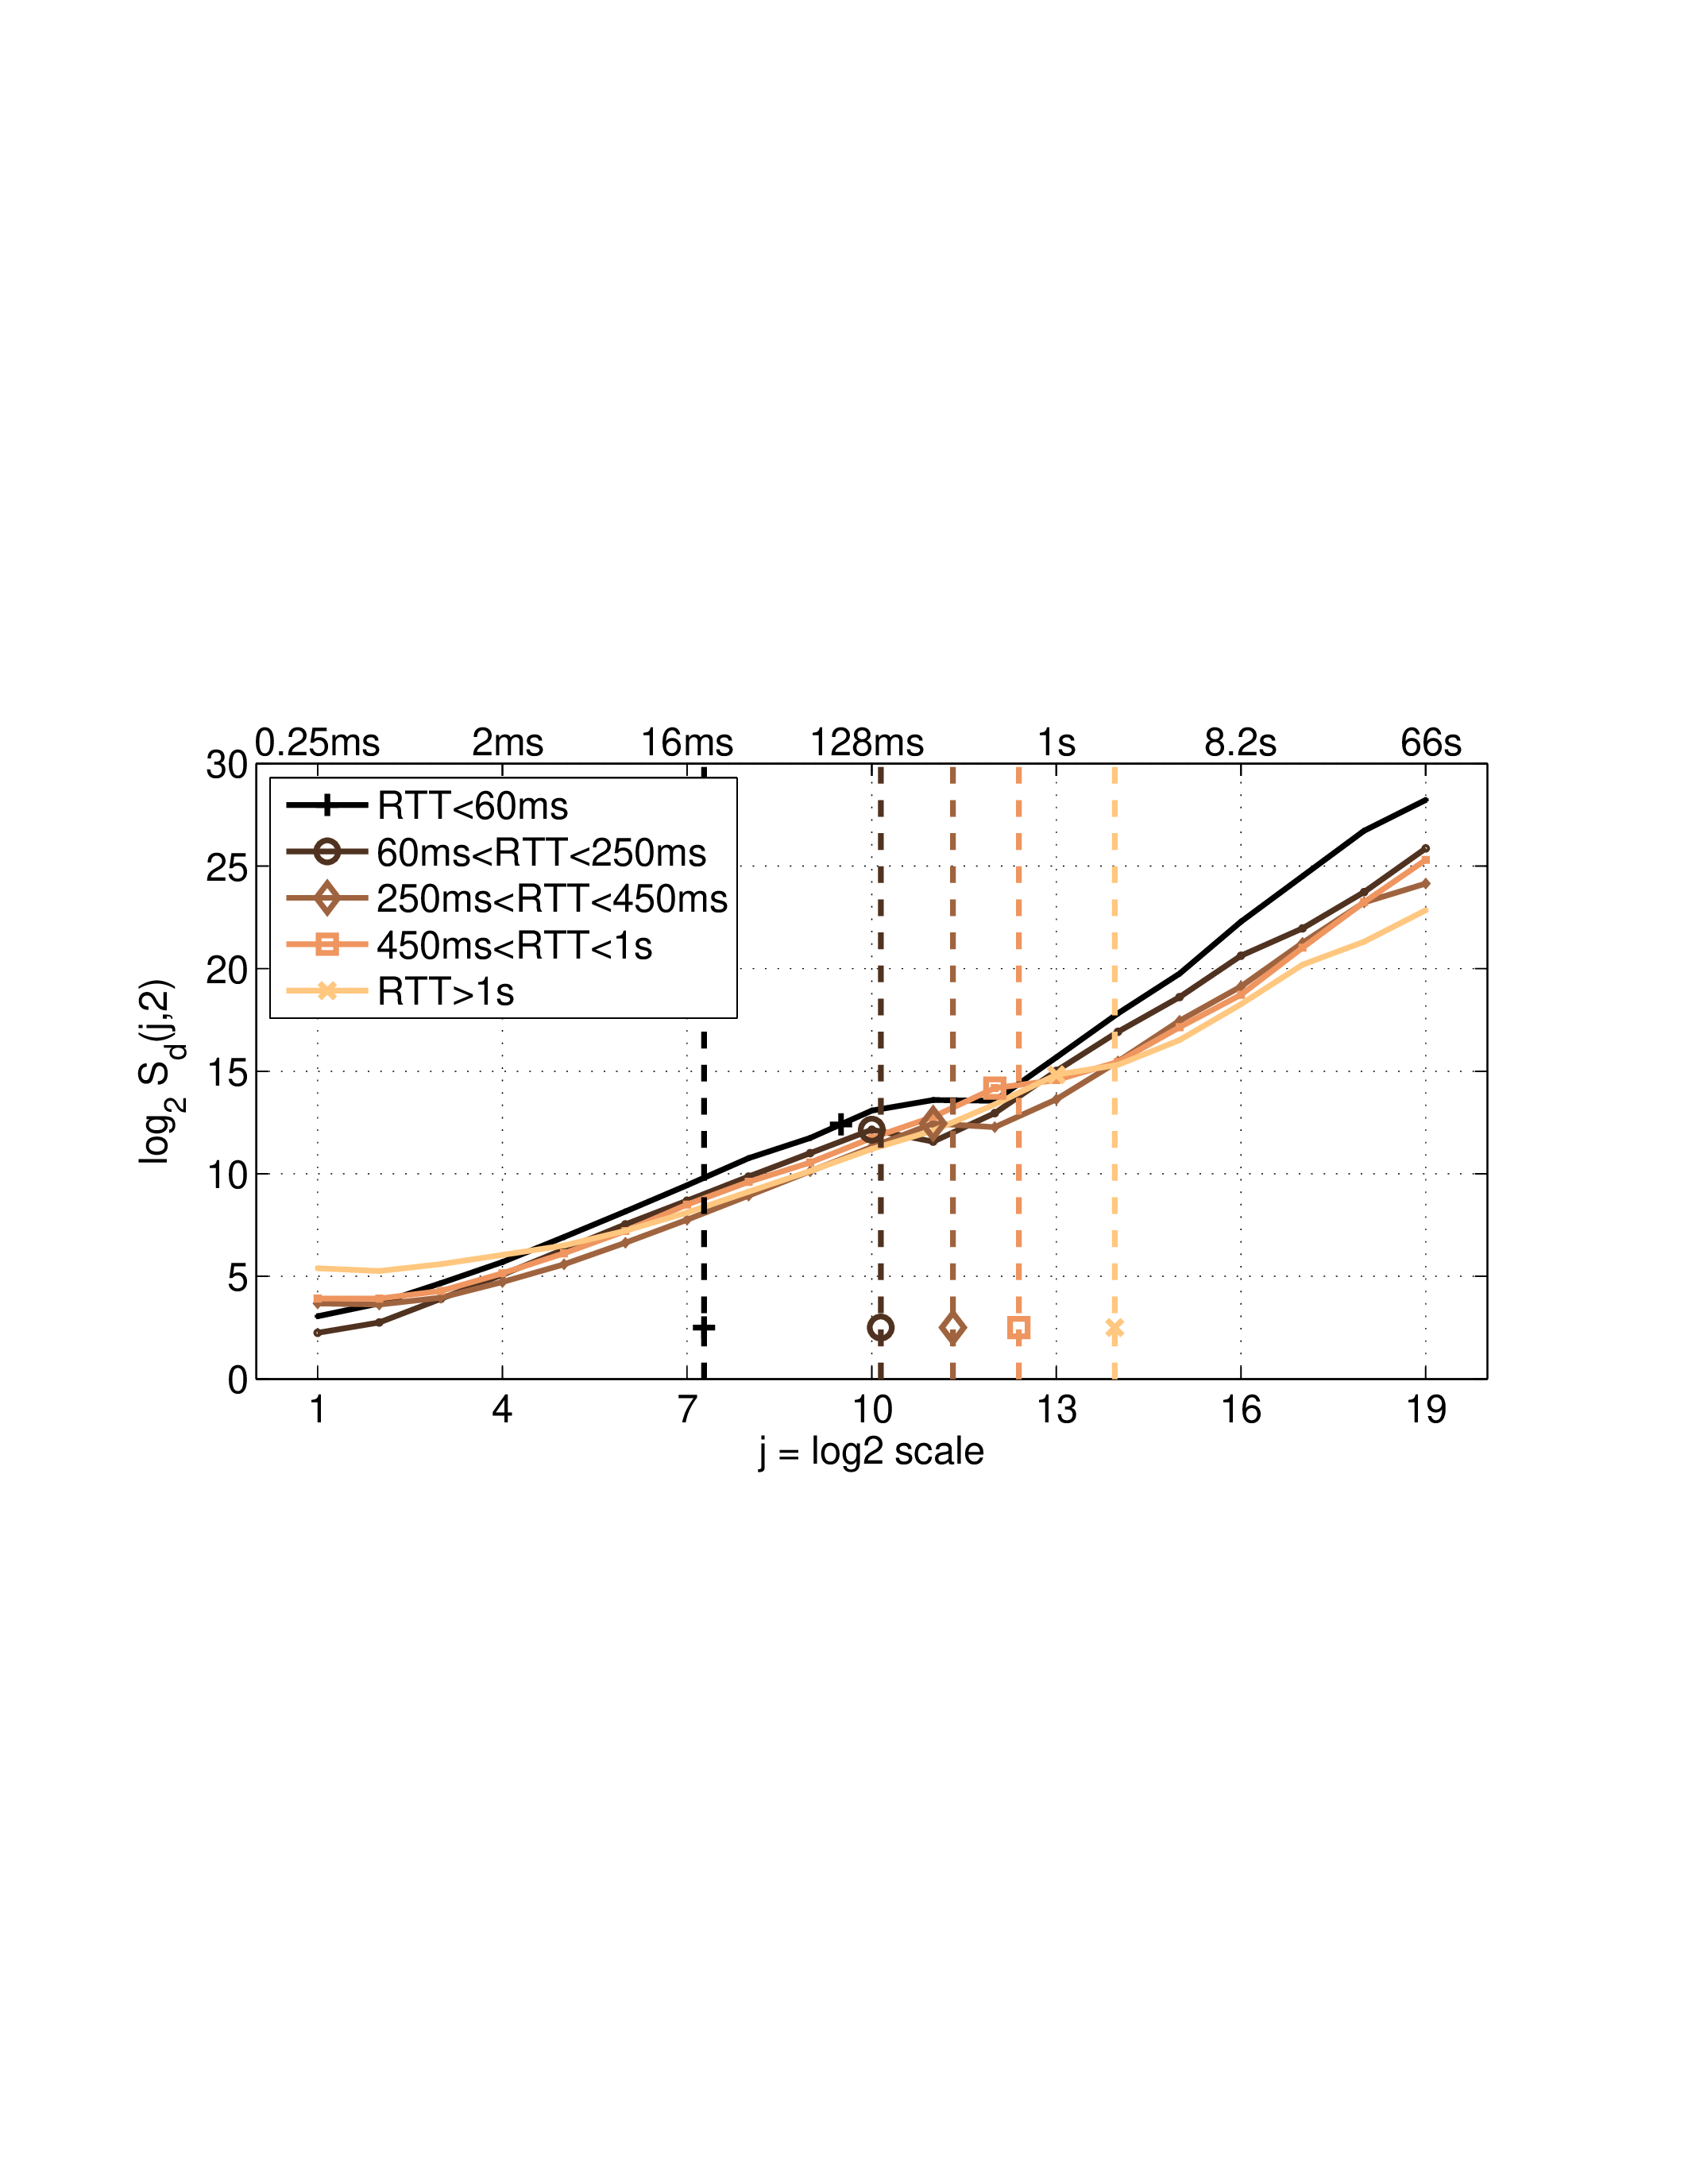}
 \includegraphics[width=.33\textwidth]{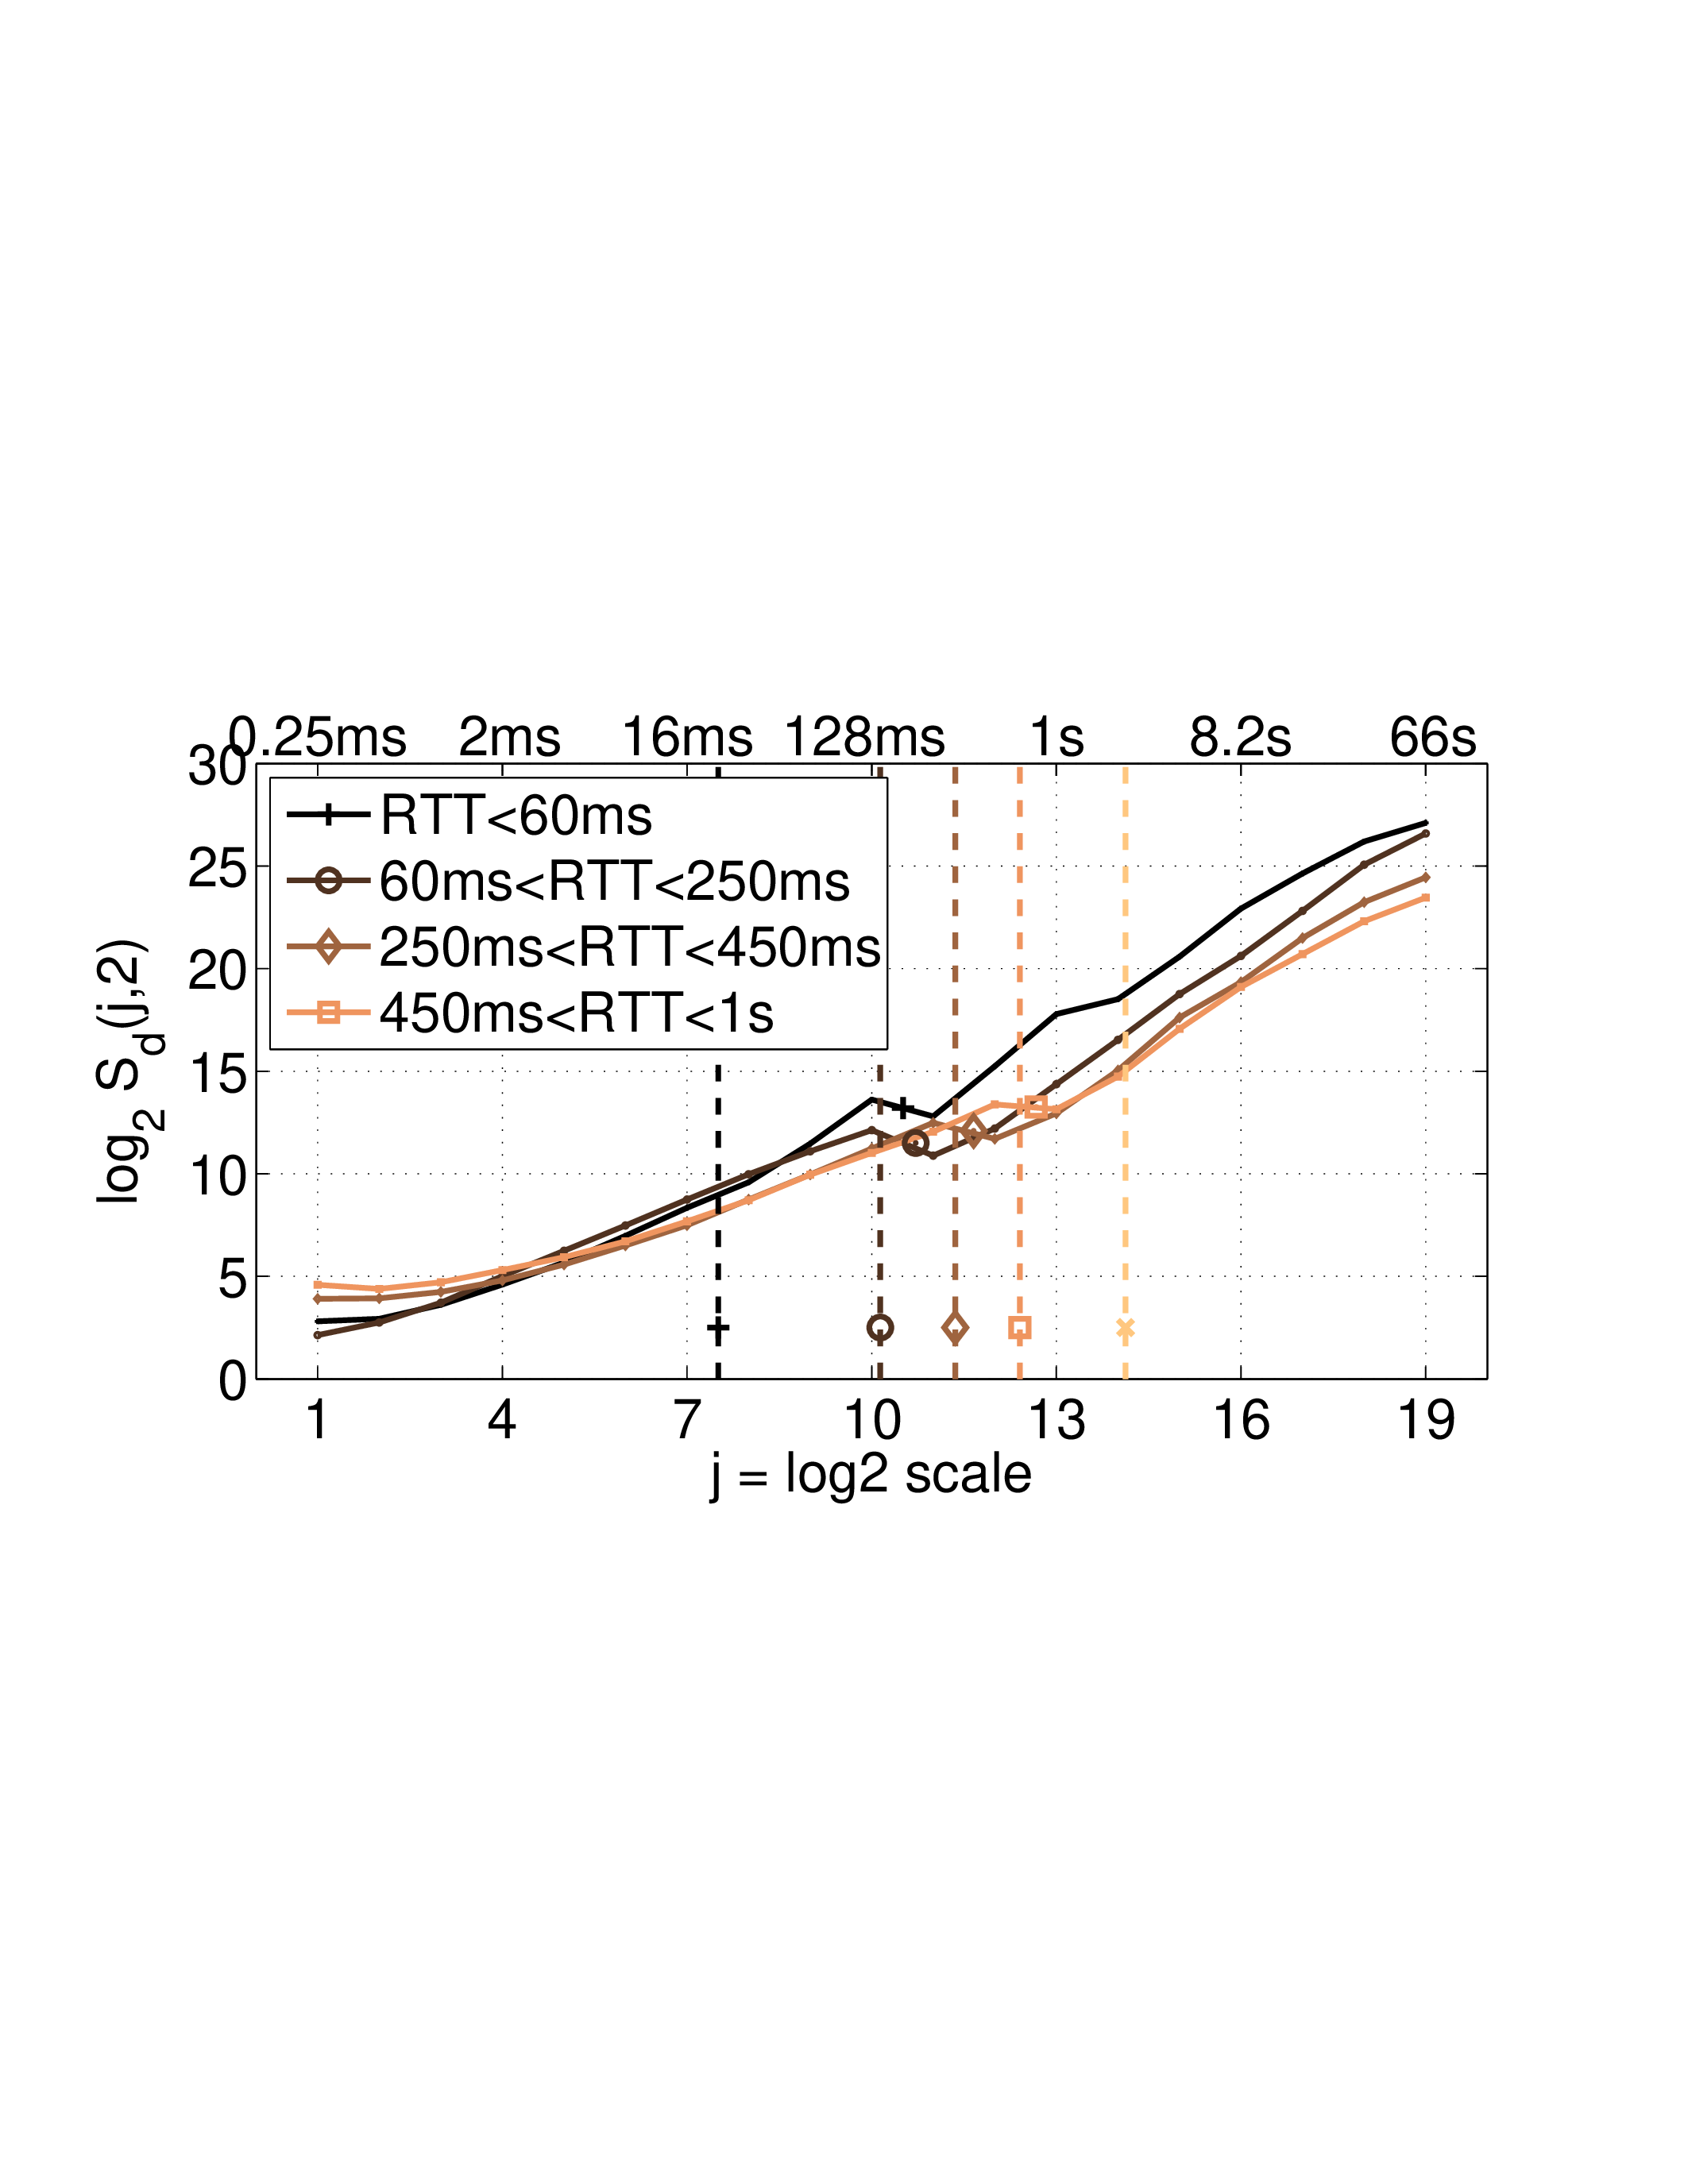}
 \includegraphics[width=.33\textwidth]{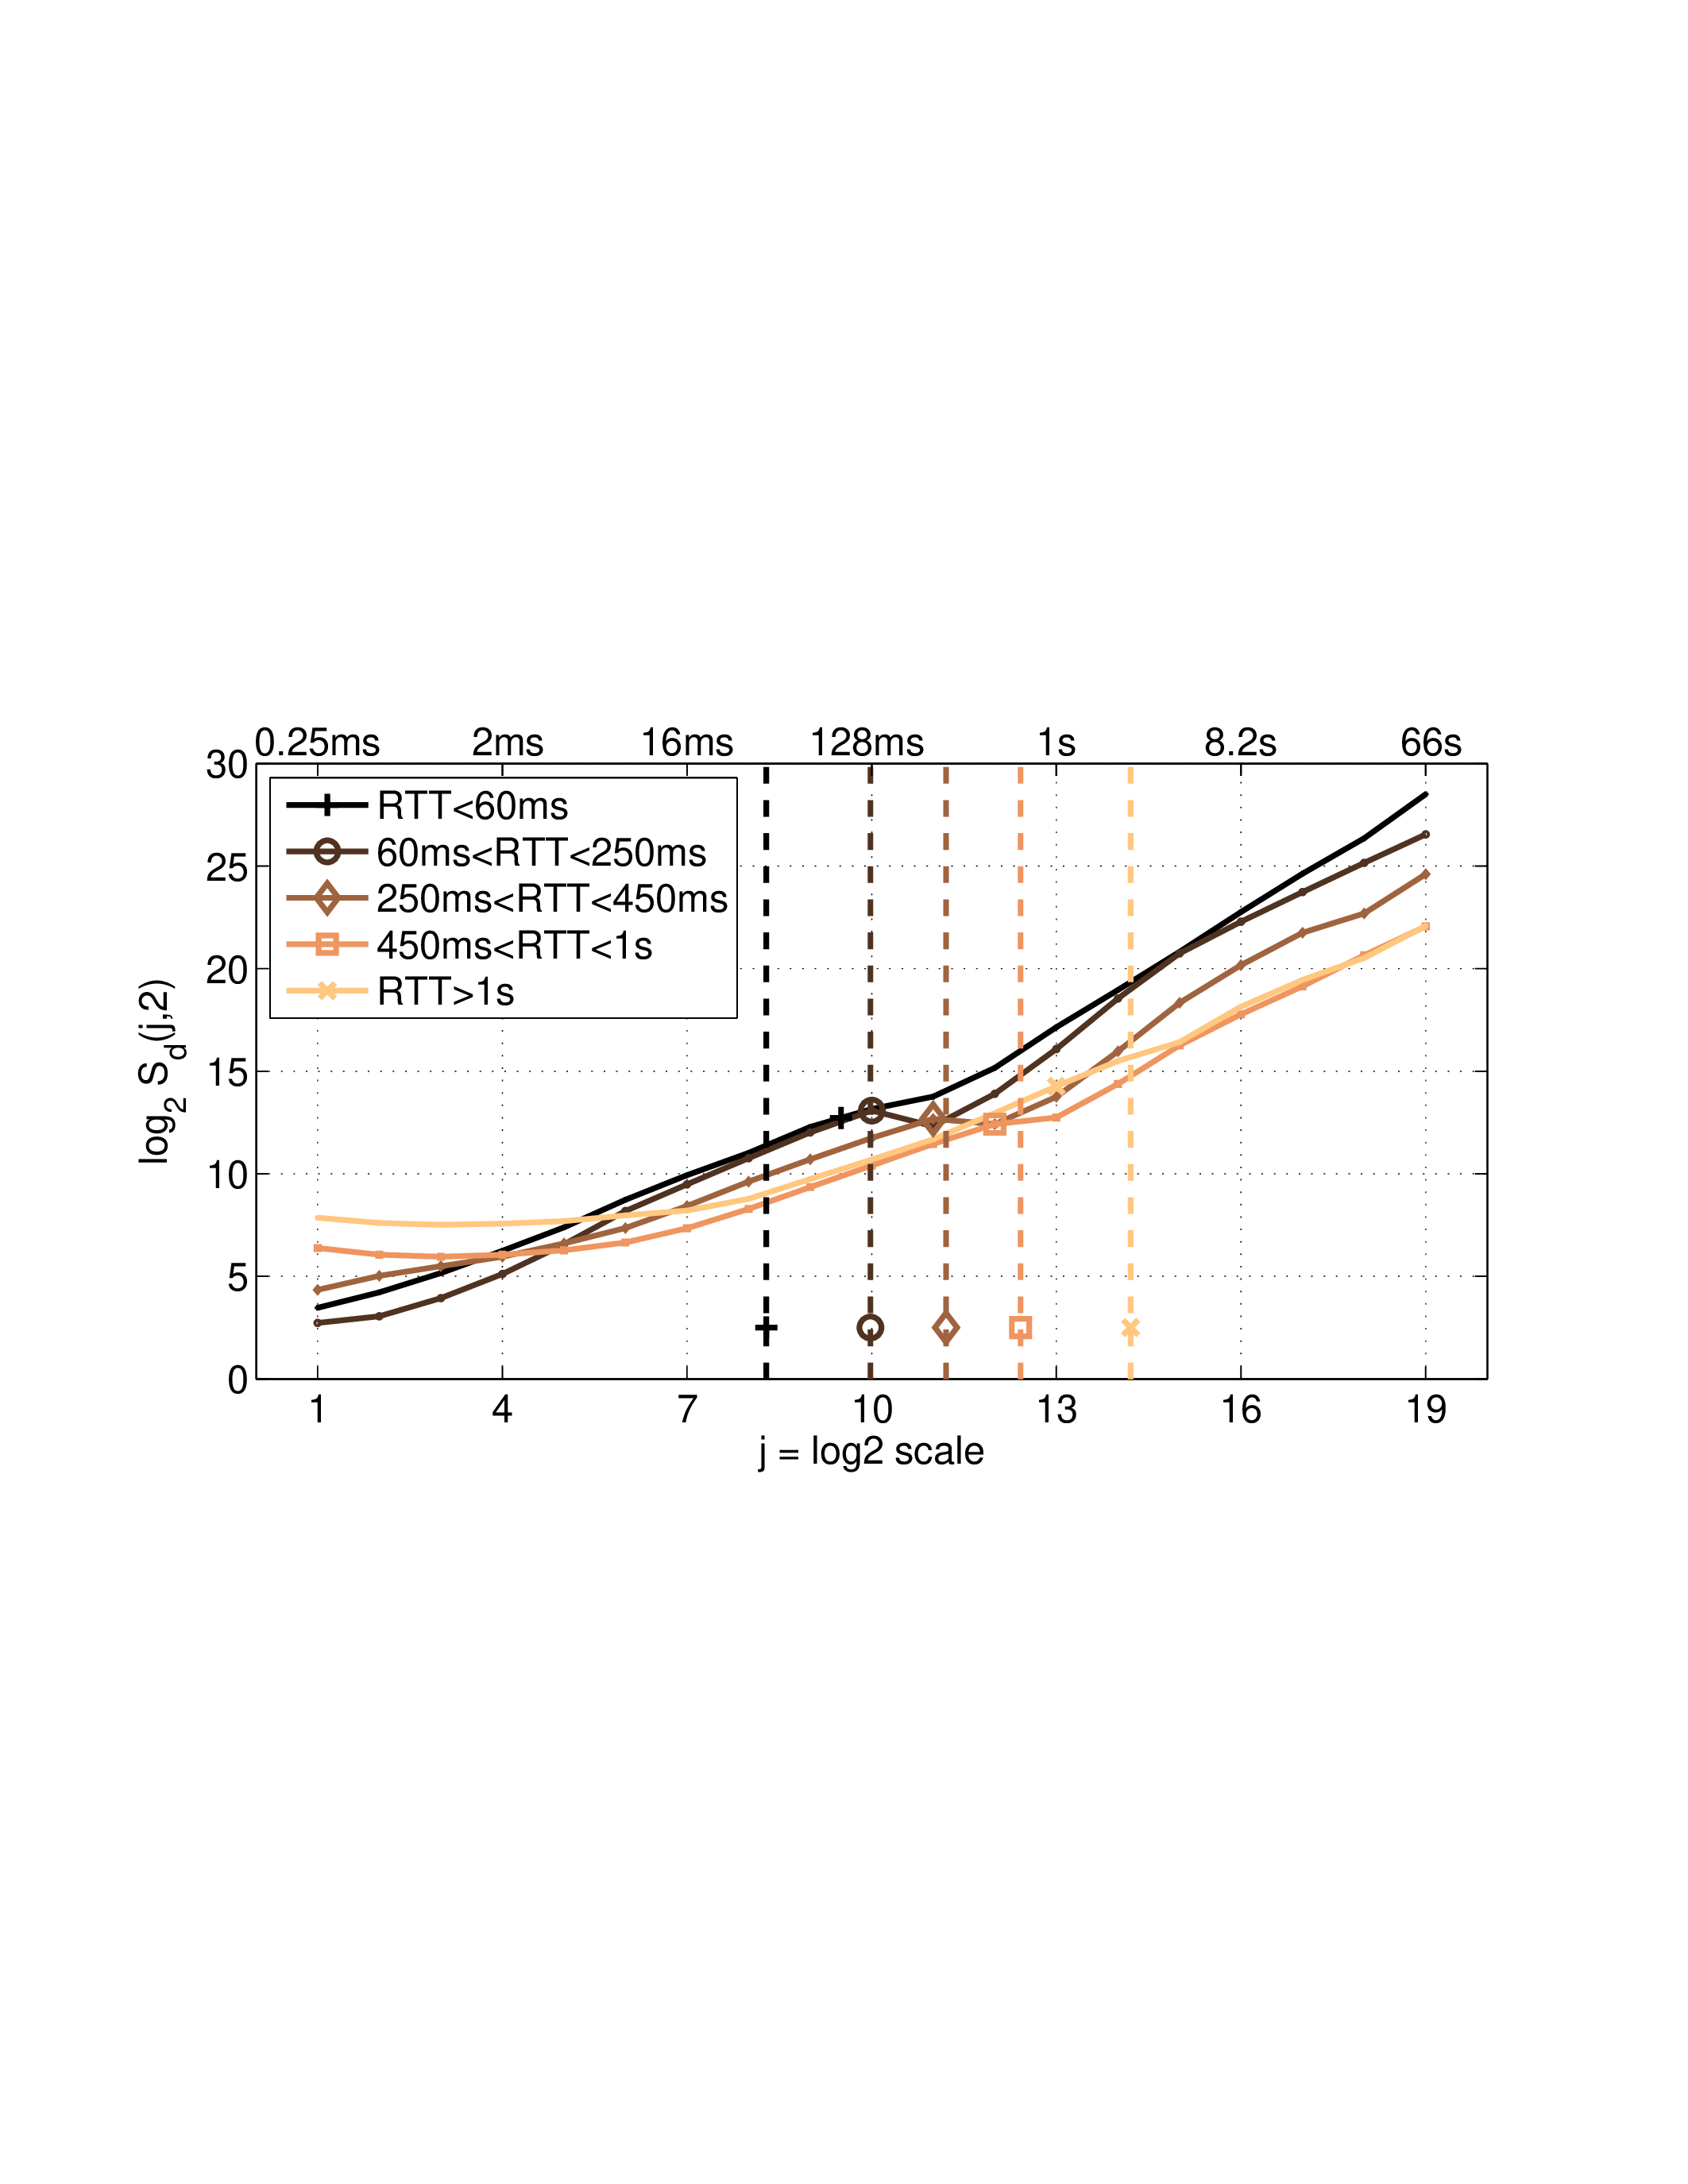}
 }
 \caption{\label{fig:LDRTT}{\bf LogScale Diagrams for three 15min-traces}, computed the median over $M=8$  sketch outputs (solid lines) for 5 sets of flows with different RTTs. The dashed-vertical lines correspond to the median RTT for each set of flows.(for comparison purpose LD are normalized). From left to right: 2009/07/06, 2011/01/03, 2013/12/07}
\end{figure*}

\begin{figure*}
\centerline{
 \includegraphics[width=0.5\linewidth]{20110103_LD_DWT_H_pkt_allMedian.eps}
  \includegraphics[width=0.5\linewidth]{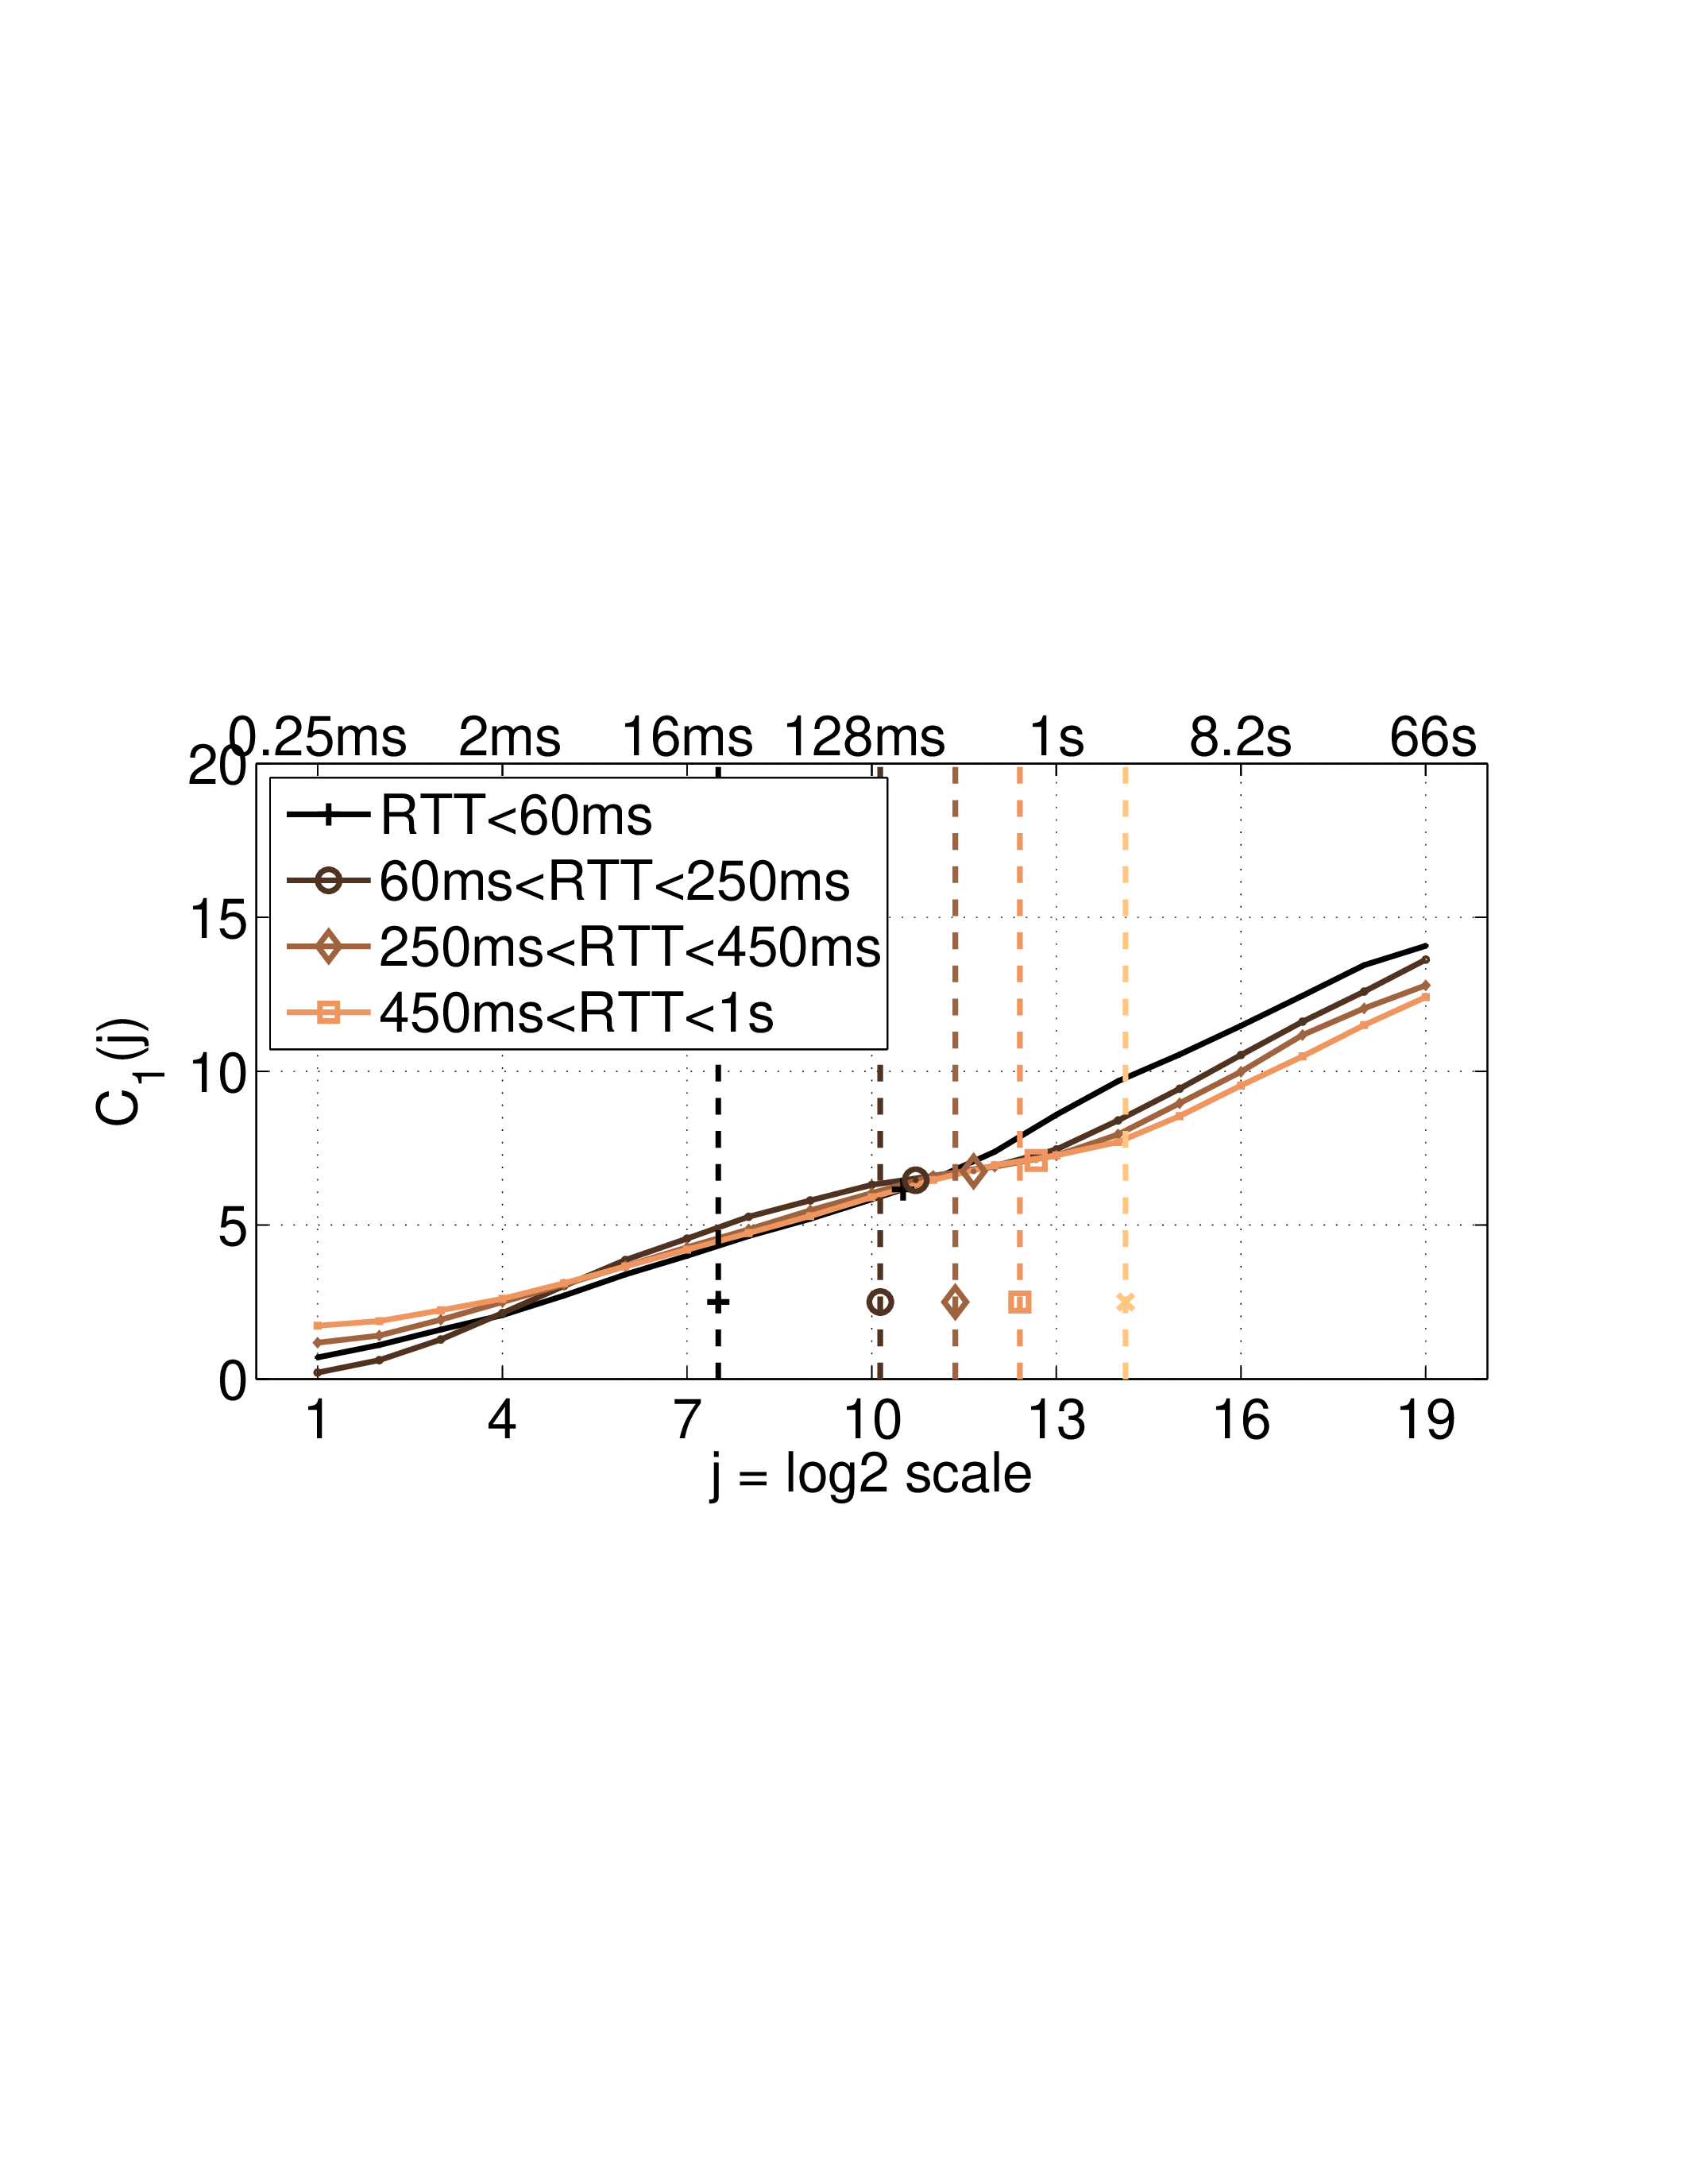}
}
\centerline{
 \includegraphics[width=0.5\linewidth]{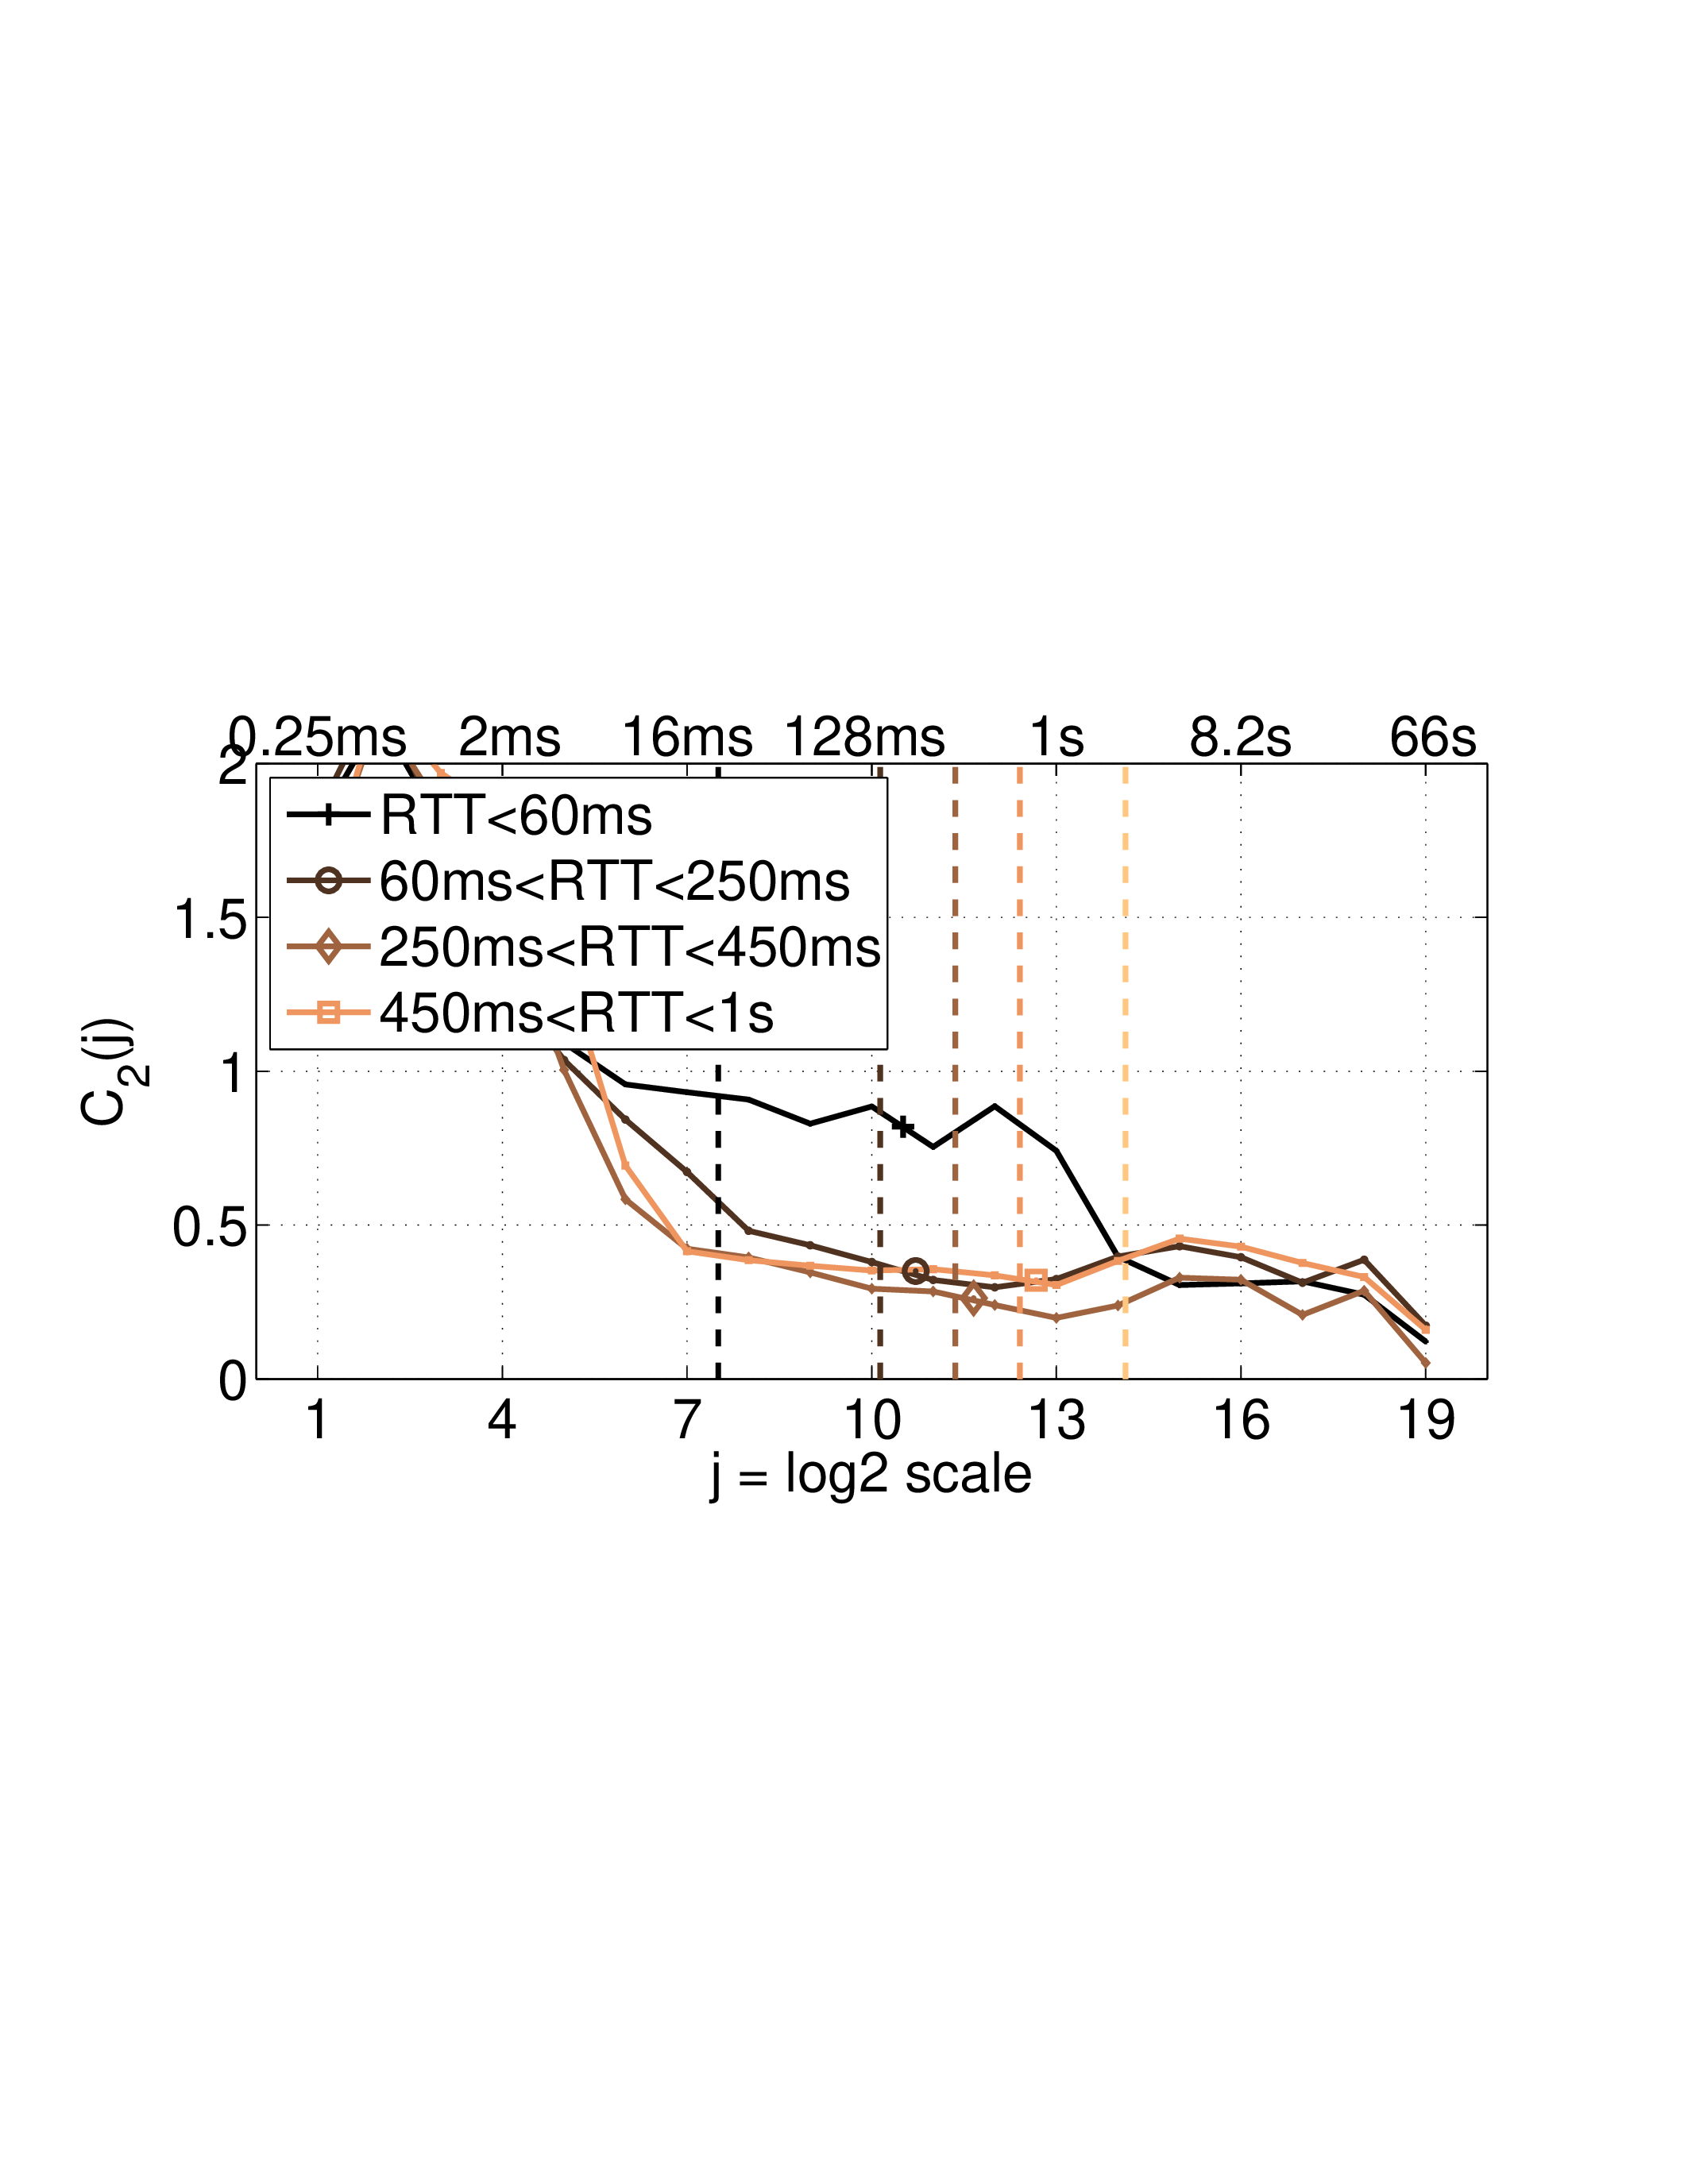}
}
\end{figure*}

\begin{figure*}
\centerline{
 \includegraphics[width=.5\linewidth]{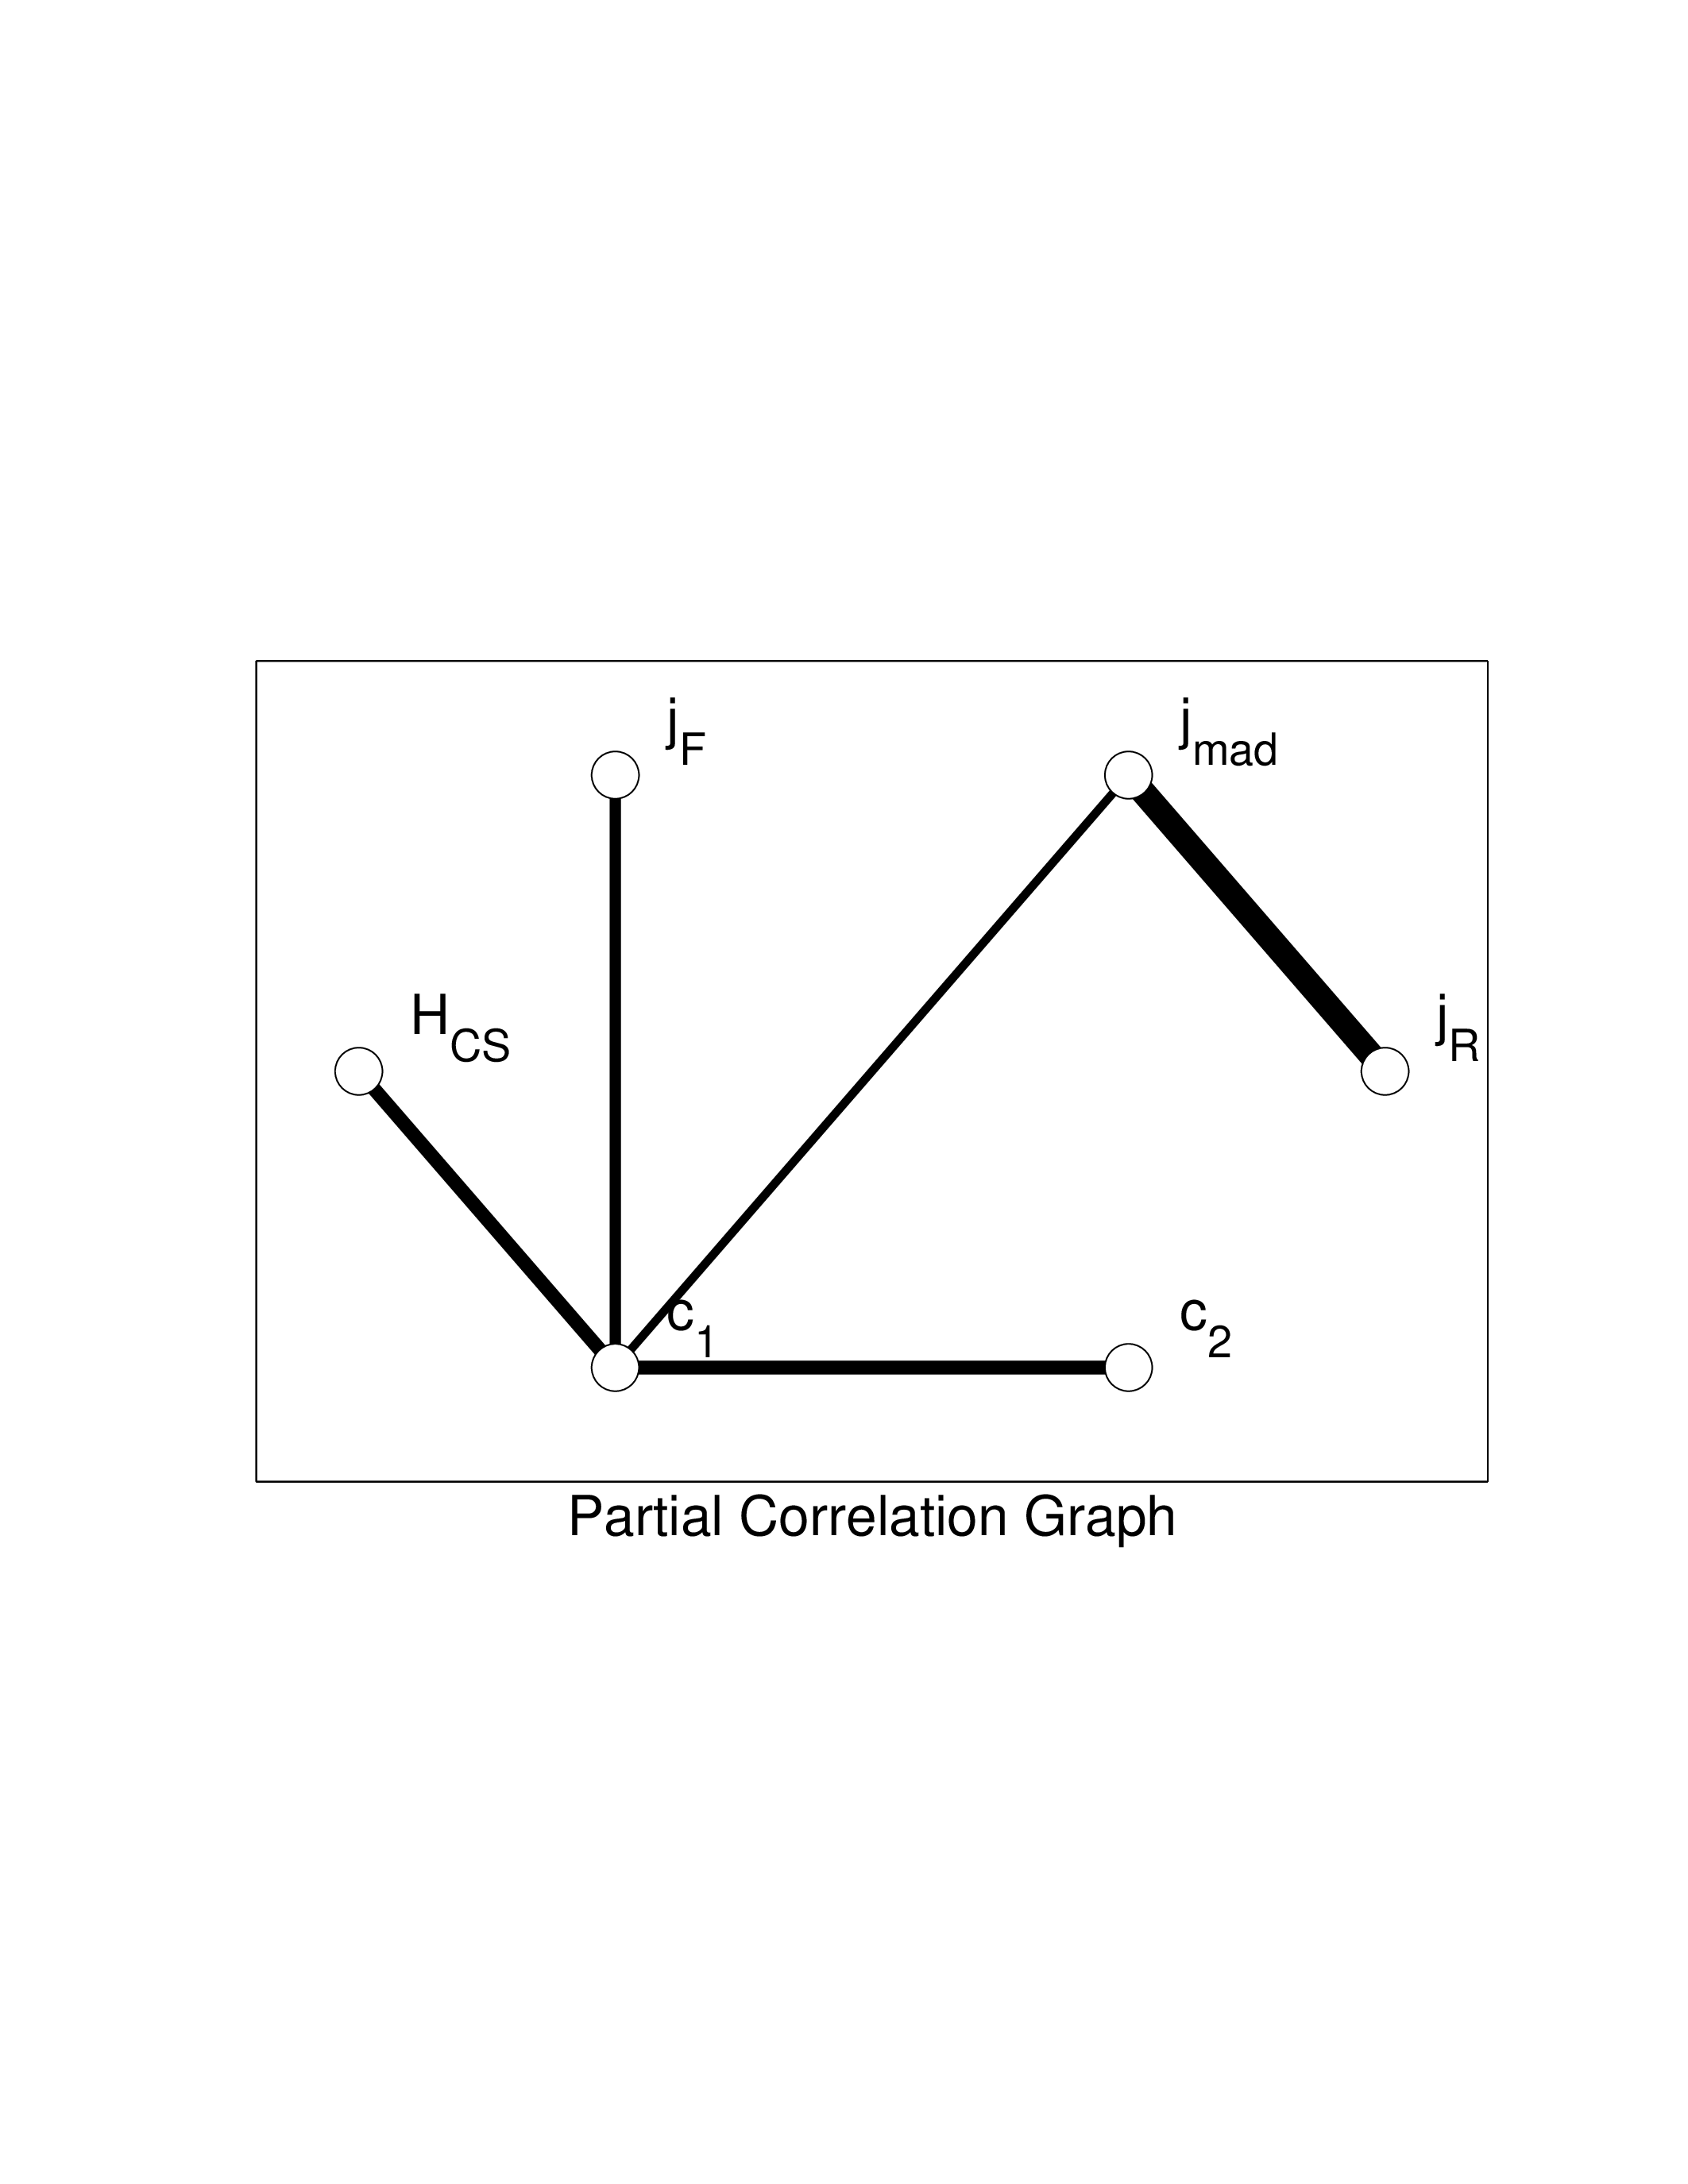}
 \includegraphics[width=0.5\linewidth]{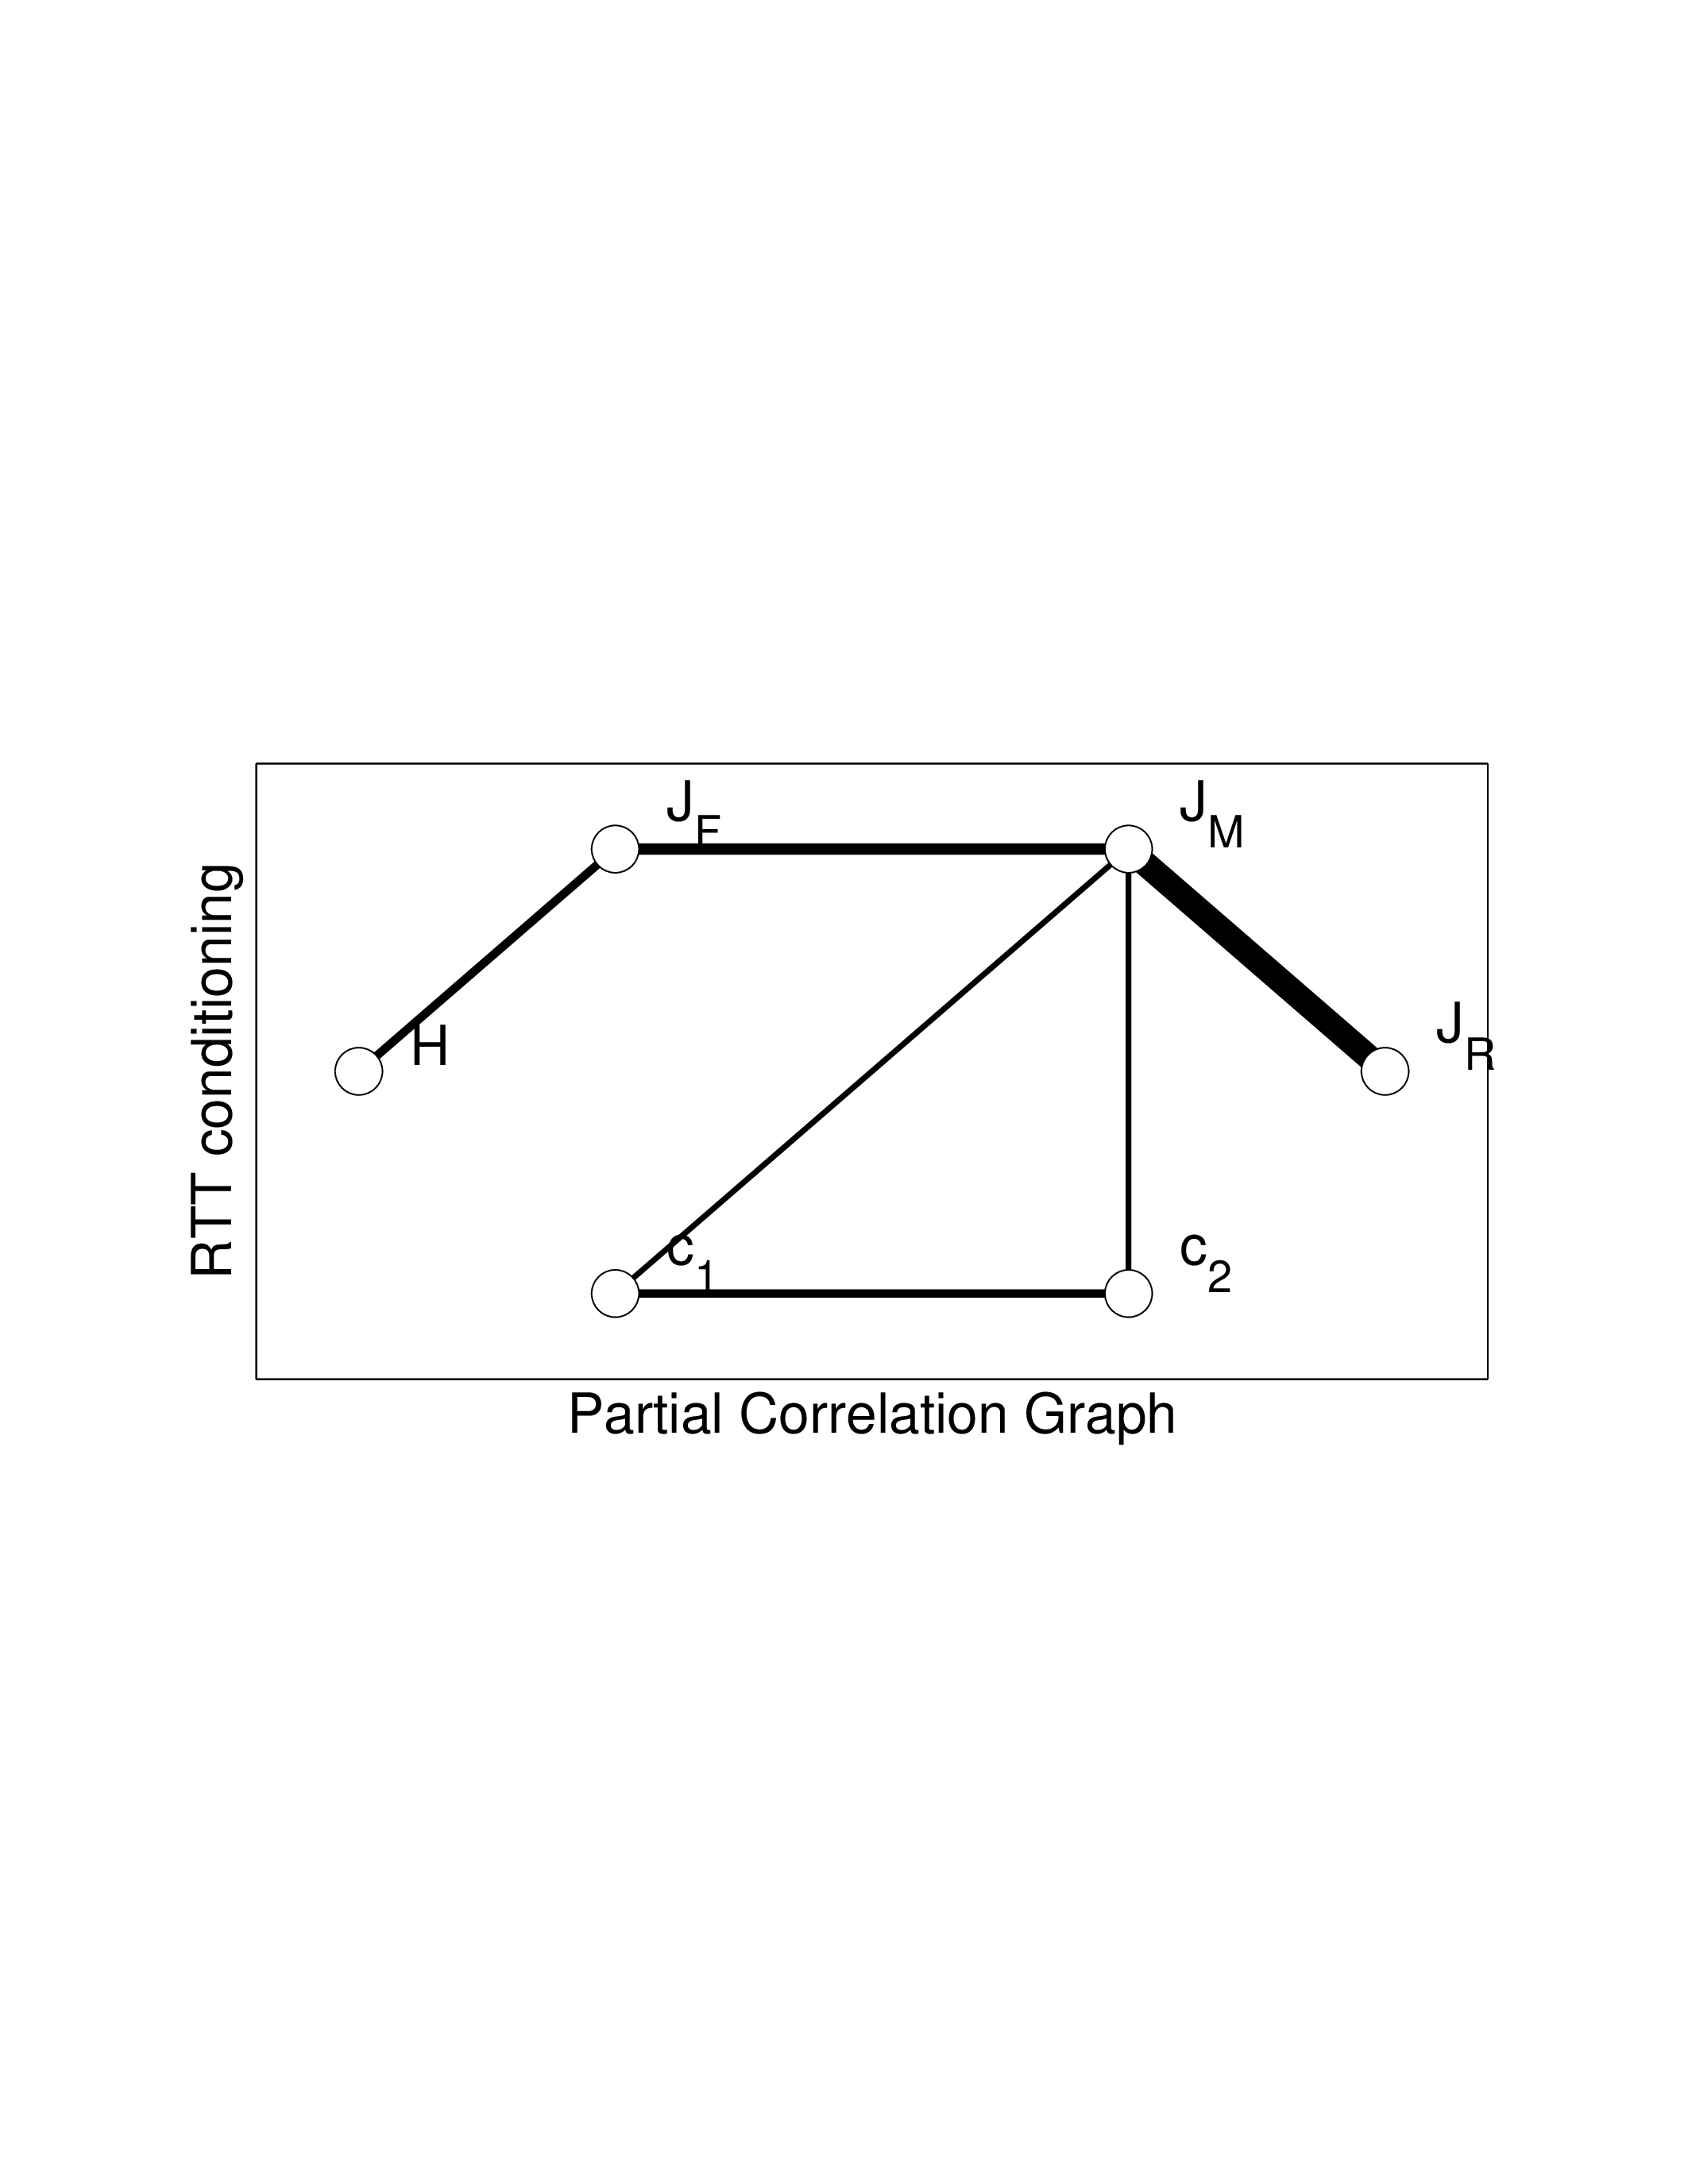}
}
\end{figure*}

\begin{table}
\begin{center}
\begin{tabular}{|l|r|r|r|r|r|r|}
\hline
                    & $j_R$ & $j_{mad}$  & $j_F$ &  $H$  &  $c_1$ &  $c_2$ \\ \hline
 $j_R$           &  -       & 0.87           & 0.27  & -0.22  & -0.32  &  0          \\ \hline
 $j_{mad}$   & -0.85 & -                &  0.34  &  -0.26 &  -0.44  &  0.19 \\ \hline
 $j_F$            &  0     &  0               & -         &   -0.16& -0.40   &   0   \\ \hline
 $H$             & 0      & 0                 &  0       & -         &  0.52 &   -0.29 \\ \hline
 $c_1$          & 0      & 0.26           & 0.31   & -0.41  & - & -0.51         \\ \hline
 $c_2$         &  0 &   0                    &  0      &  0       & 0.44  & -            \\ \hline
\end{tabular}
\end{center}
\caption{\label{tab:partial} {\bf Correlations.} Direct (upper right triangle) and partial (lower left triangle) correlations. The corresponding partial correlation graph is depicted in Fig.~\ref{fig:Halpha} (left).}
\end{table}
